# Supplementary material for: Attention Deficit is Ordered! Fooling Deformable Vision Transformers with Collaborative Adversarial Patches
Source: arXiv:2311.12914 source file (2023-12-25)
Supplement: Supplementary file 1 [file 7_supplementary.tex]

\section{Code}
The code is provided as part of the supplementary material. Upon acceptance of the paper, the code will be made public 
in the anonymous Github repository mentioned in the Introduction. The provided README.md file contains all the required information to setup the environment and run the code.

\section{Illustration of attack on DeTr}
\subsection{Perceptibly of the patches}
When the adversarial patch is placed on the test images, the patch can be barely discovered in the resulting images. The patch may be perceived as a faint camera flicker, or a small printed sign on a surface (e.g., T-shirt or signboard). Fig. \ref{fig:comparison} shows two instances of clean and patched image-pairs, with a source patch at (400, 400) and a target patch at (100, 100). In this experiment, we took two 32x32 patch, but this attack can be realized with a 16x16 or even a 8x8 patch, making the patches almost imperceptible.
\begin{figure}[h]
    \centering
    \begin{subfigure}[b]{0.9\linewidth}
        \includegraphics[width=\textwidth]{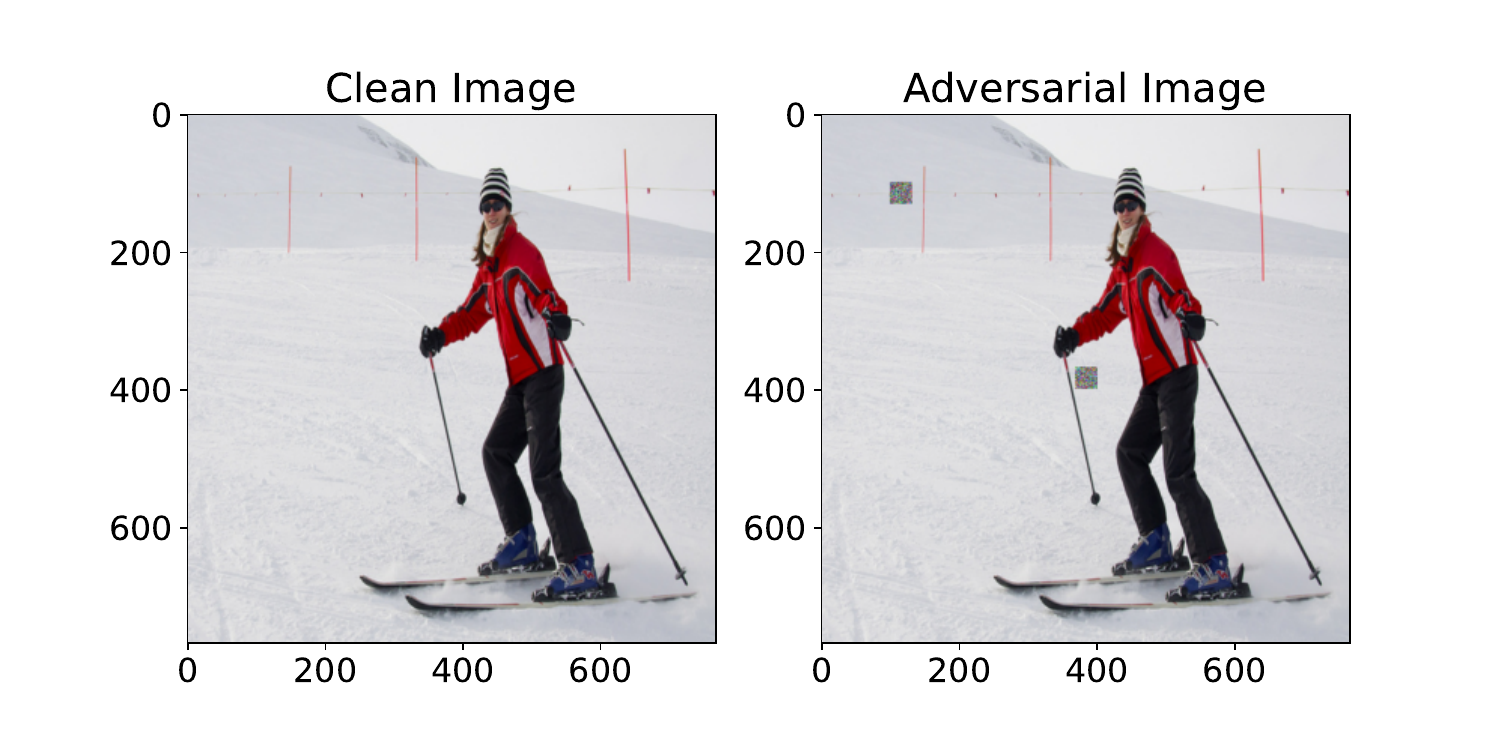}
        \label{fig:noticable}
    \end{subfigure}
    \vspace{-15pt}
    \begin{subfigure}[b]{0.9\linewidth}
        \includegraphics[width=\textwidth]{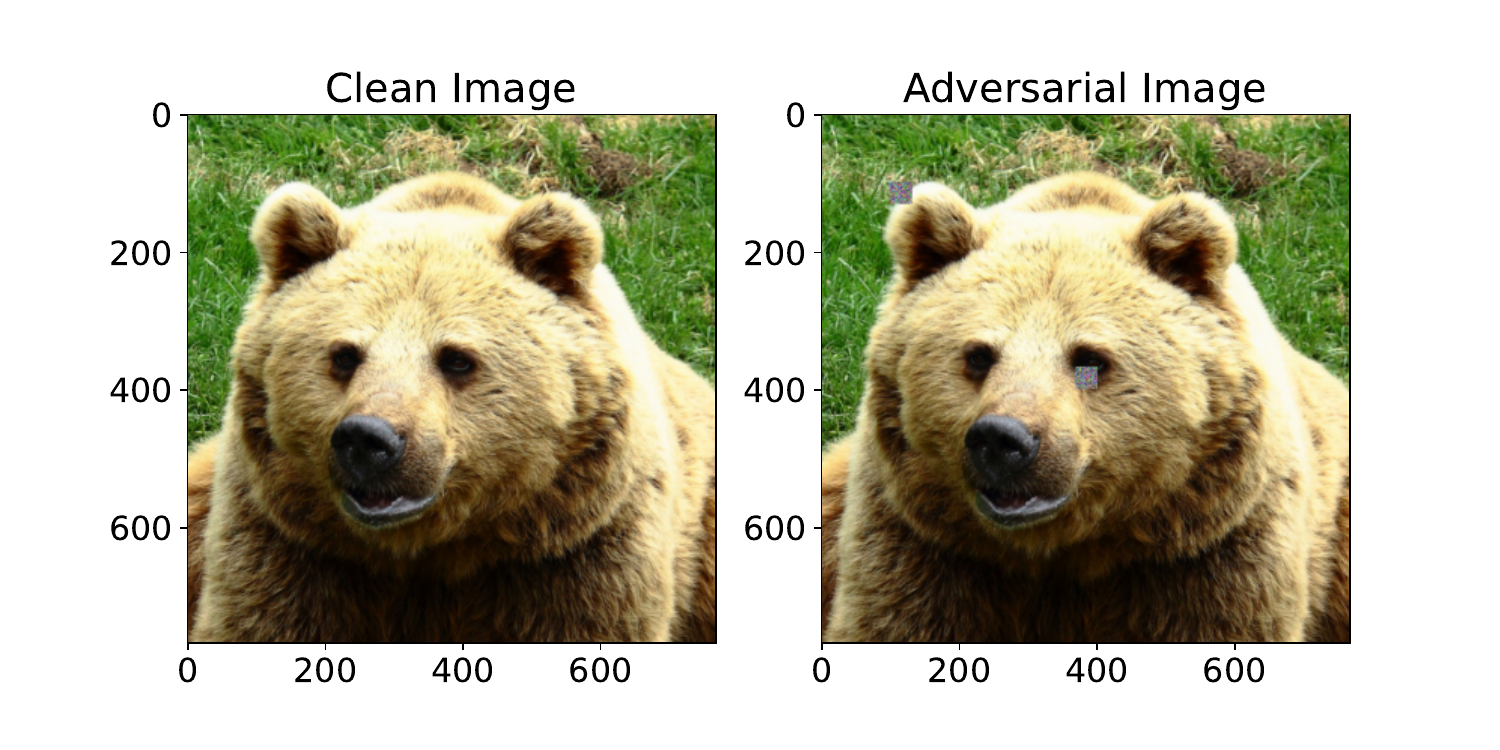}
        \label{fig:unnoticable}
    \end{subfigure}
    \caption{Comparison of clean and adversarial images. The patches are more noticeable in the images with clear background, but in the most common case they can be hardly perceptible.}
    \label{fig:comparison}
\end{figure}

\subsection{Change in bounding-box results}
The patches generated by all four attacks (i.e., IP, OP, SP, CP) has catastrophic effect on the bounding-box results. In the detection results on patched images, in most cases bounding-boxes are absent (no objects found). In Fig. \ref{fig:bbox_IP}, \ref{fig:bbox_OP}, \ref{fig:bbox_SP}, and \ref{fig:bbox_CP}, examples of bounding-box annotation results are presented for clean and patched images, alongside their corresponding ground-truth, illustrating instances of IP, OP, CP, and SP attacks, respectively.

\begin{figure*}[t] % Use the star (*) to span both columns
    \centering
    \begin{minipage}{\textwidth}
        \includegraphics[width=\linewidth]{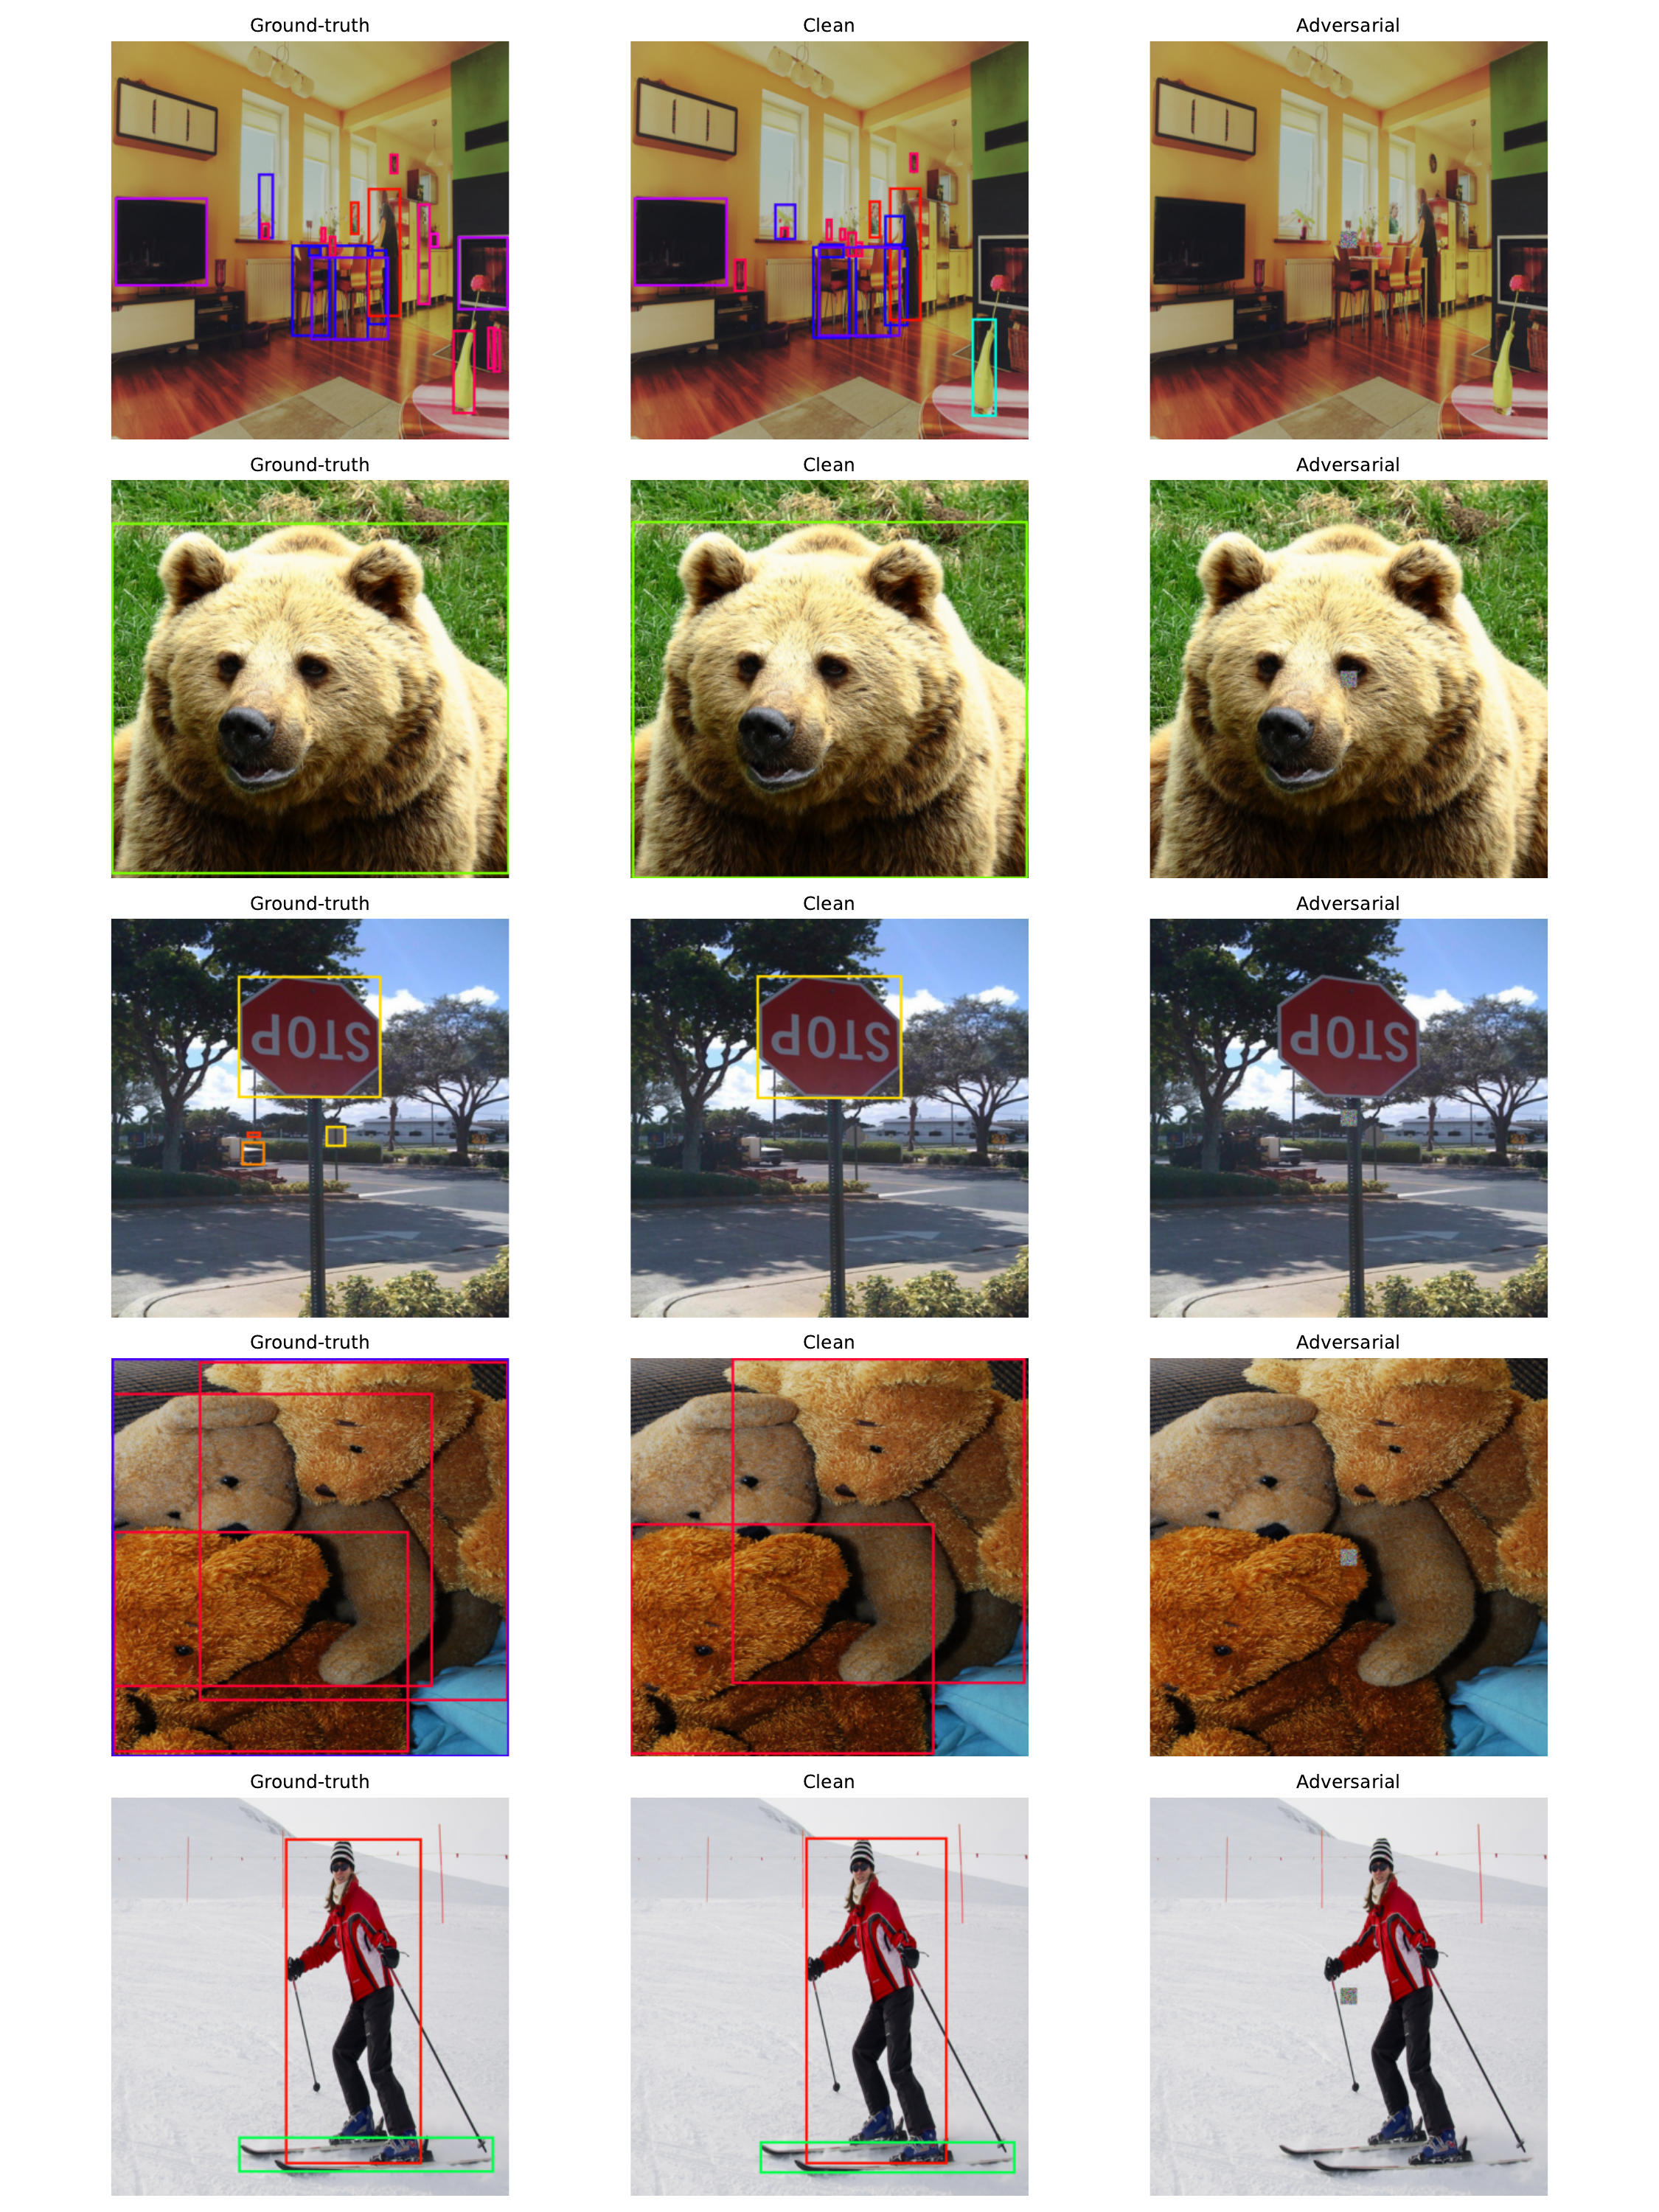}
        \caption{Bounding box comparison among ground-truth, clean images, and adversarial images in IP attack.}
        \label{fig:bbox_IP}
    \end{minipage}
\end{figure*}

\begin{figure*}[t] % Use the star (*) to span both columns
    \centering
    \begin{minipage}{\textwidth}
        \includegraphics[width=\linewidth]{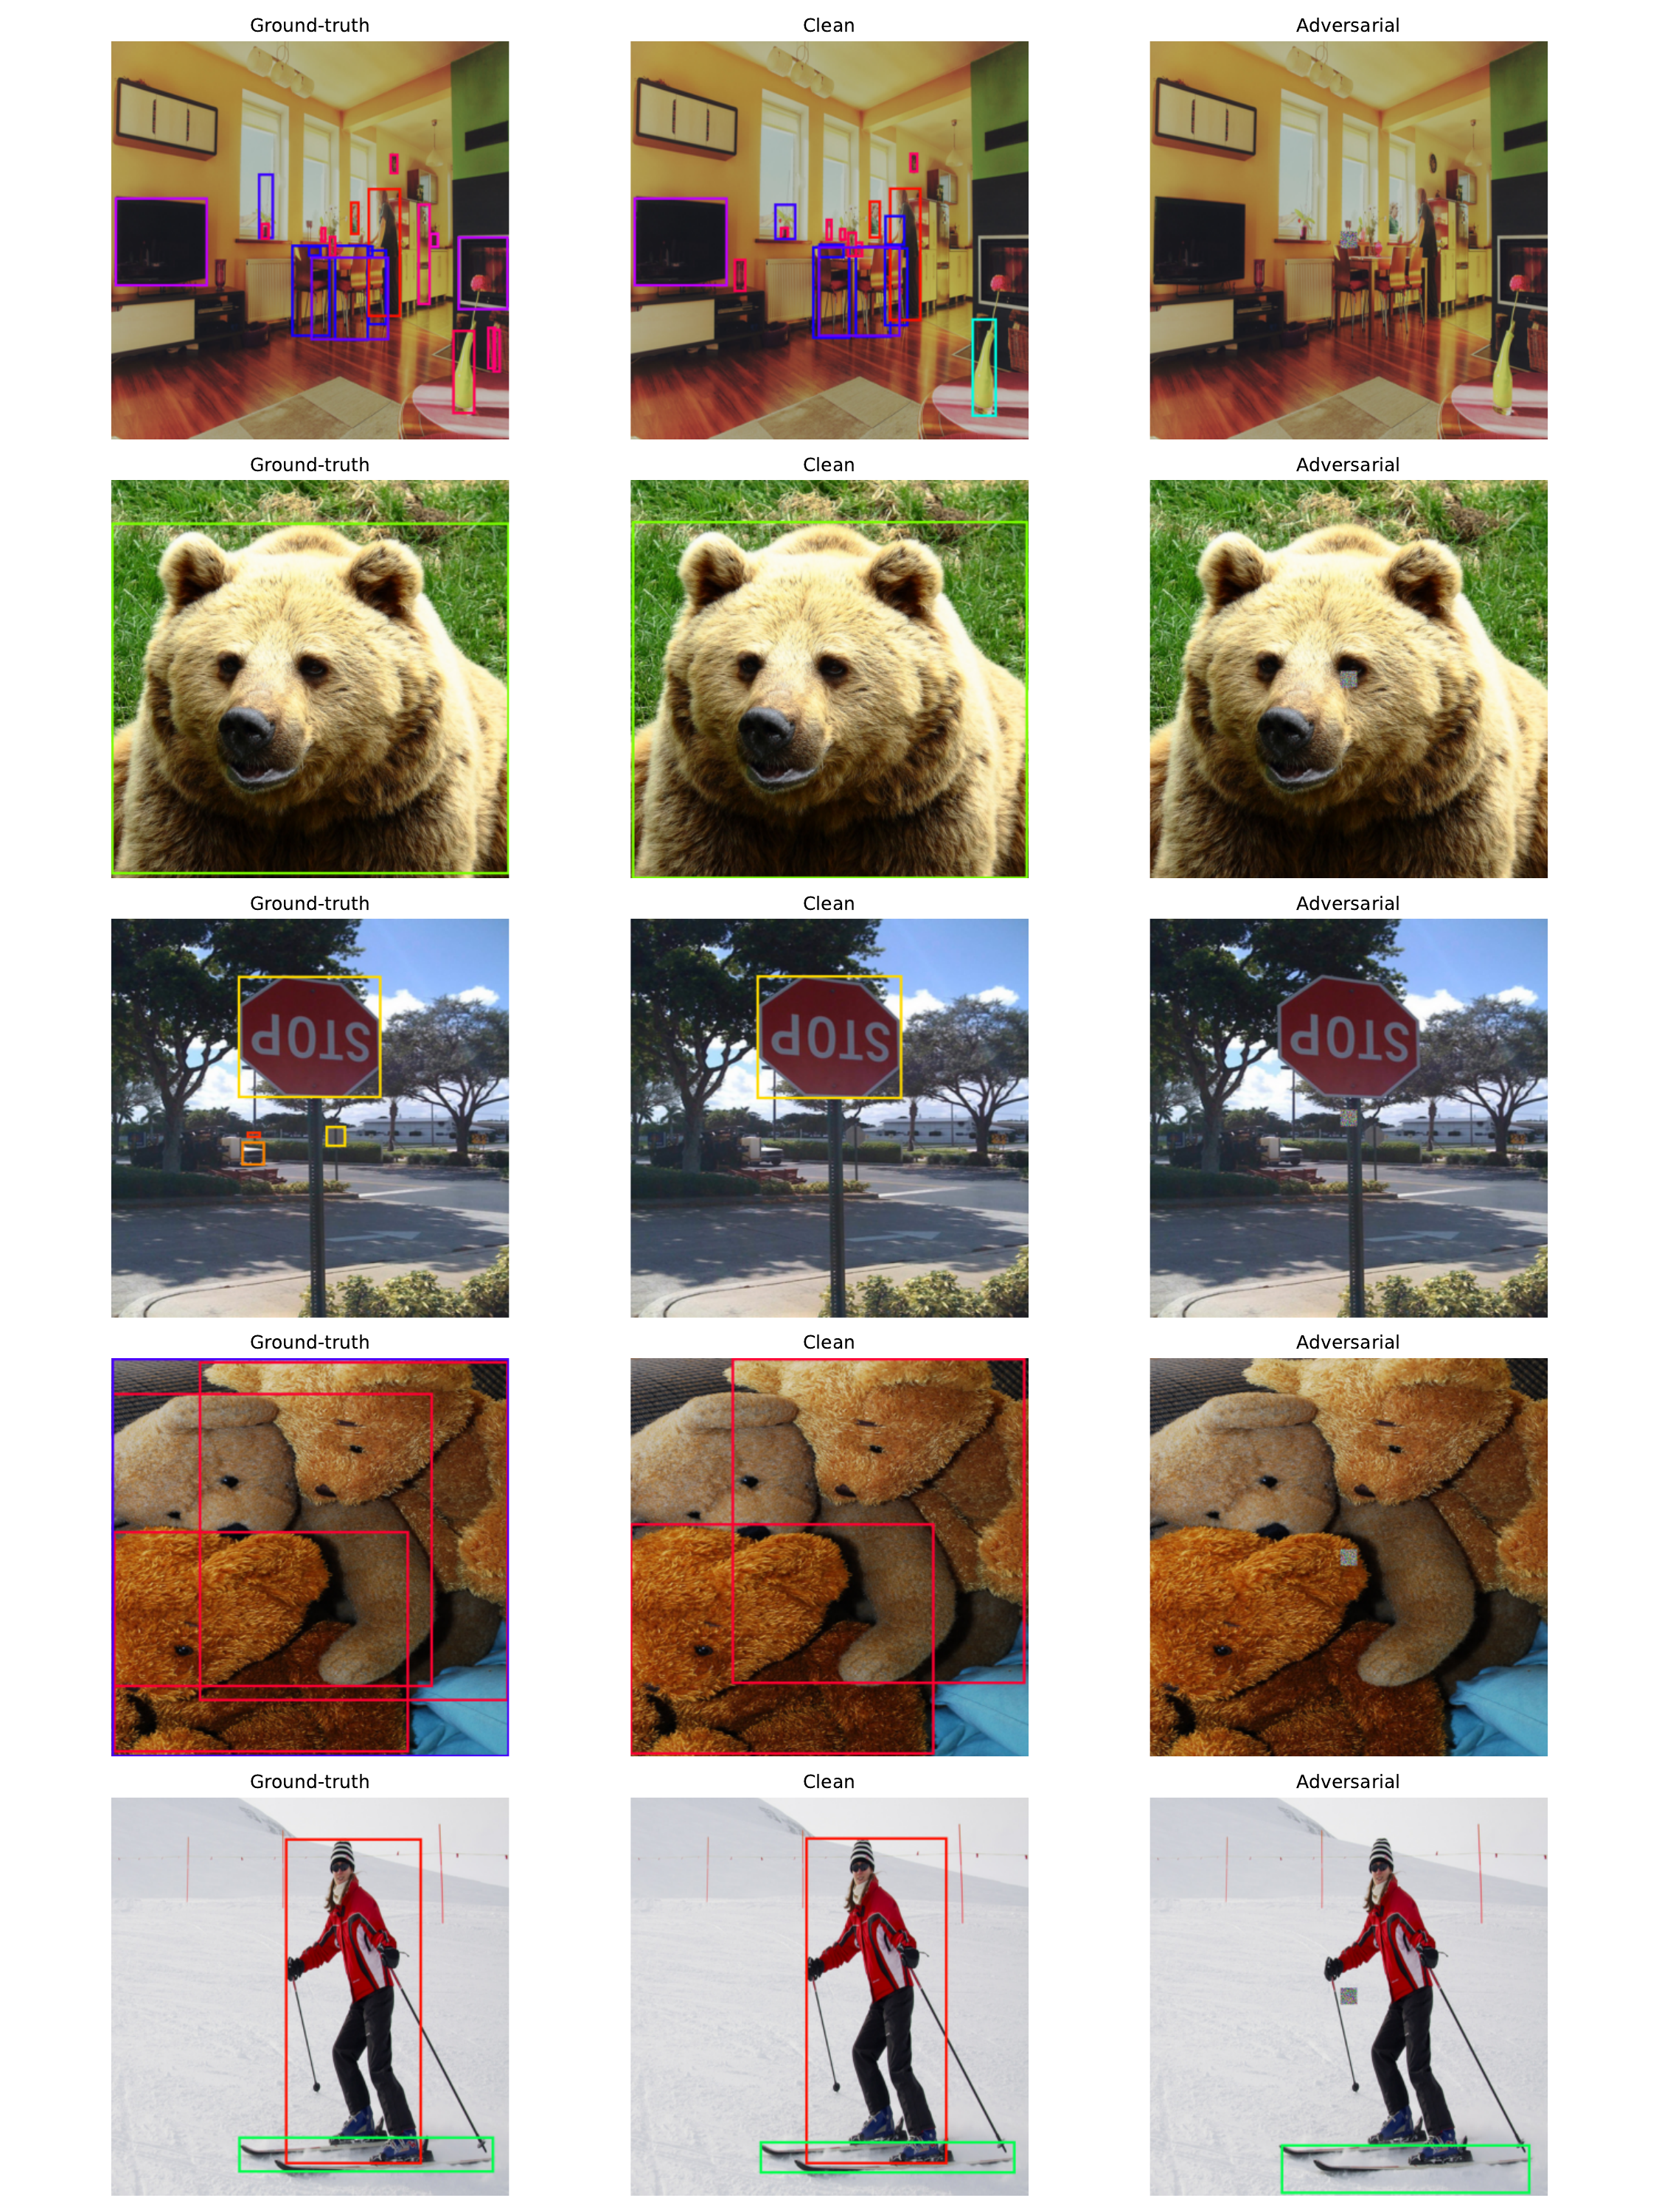}
        \caption{Bounding box comparison among ground-truth, clean images, and adversarial images in OP attack.}
        \label{fig:bbox_OP}
    \end{minipage}
\end{figure*}

\begin{figure*}[t] % Use the star (*) to span both columns
    \centering
    \begin{minipage}{\textwidth}
        \includegraphics[width=\linewidth]{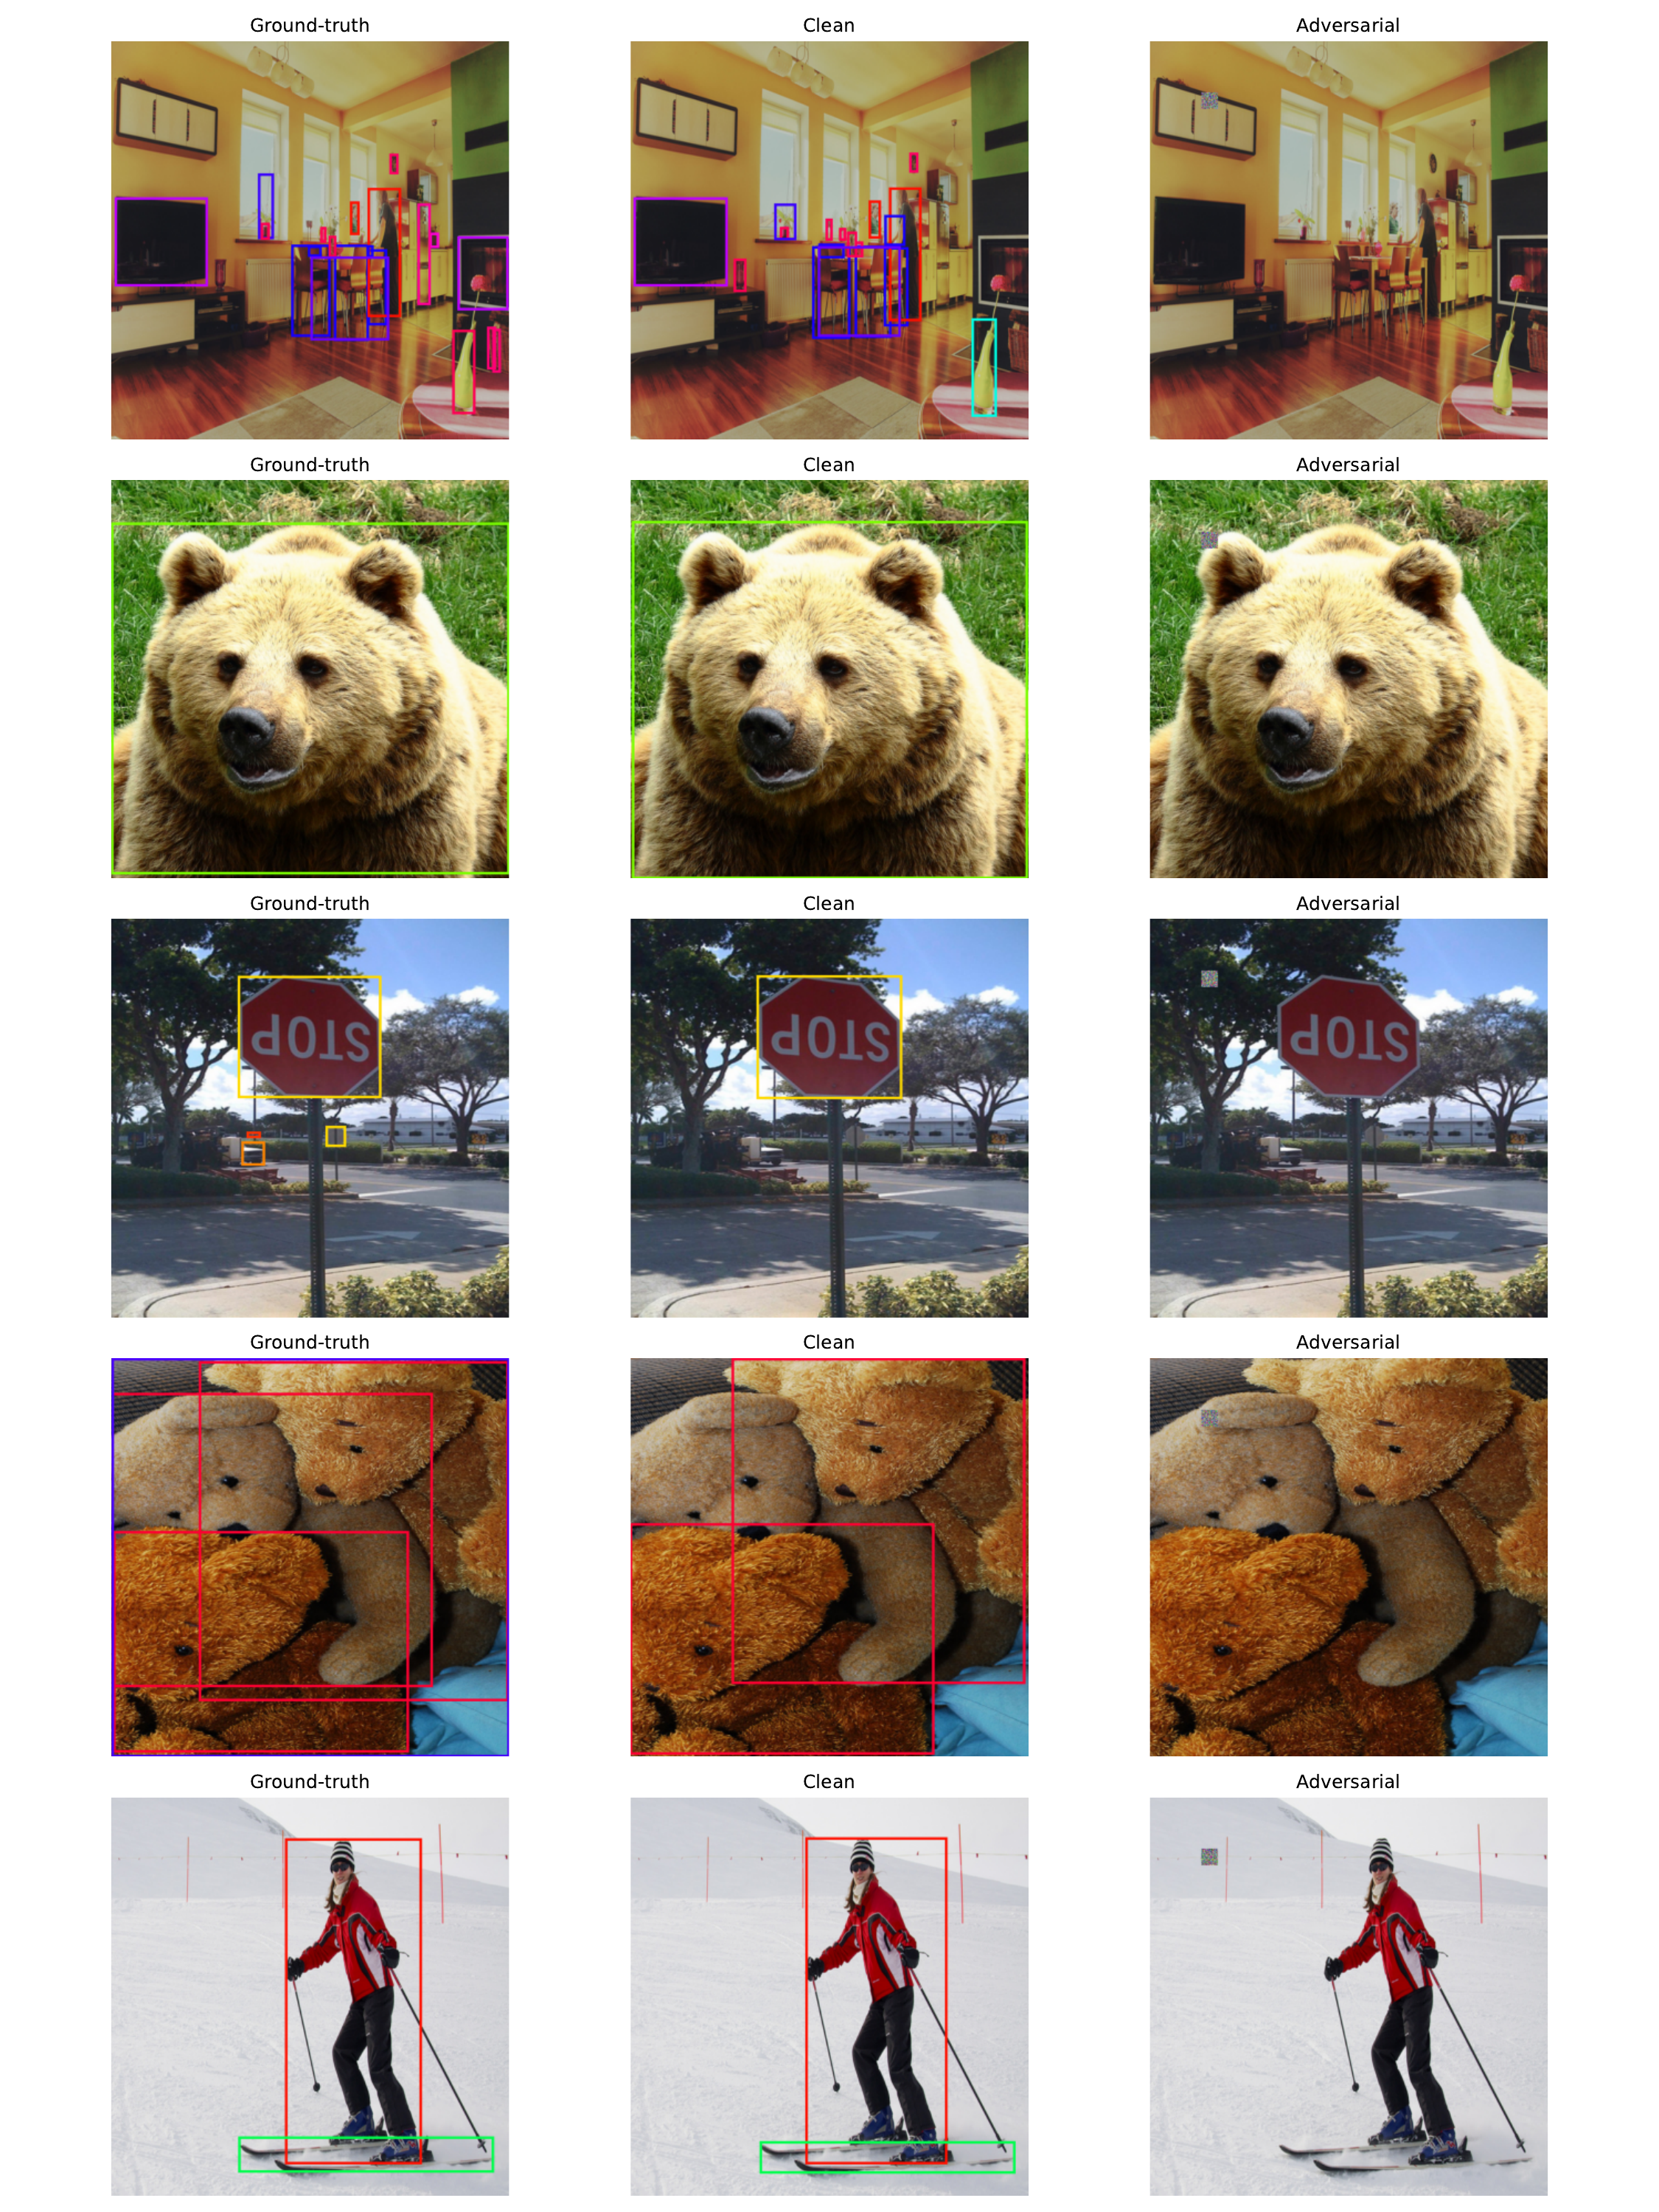}
        \caption{Bounding box comparison among ground-truth, clean images, and adversarial images in SP attack.}
        \label{fig:bbox_SP}
    \end{minipage}
\end{figure*}

\begin{figure*}[t] % Use the star (*) to span both columns
    \centering
    \begin{minipage}{\textwidth}
        \includegraphics[width=\linewidth]{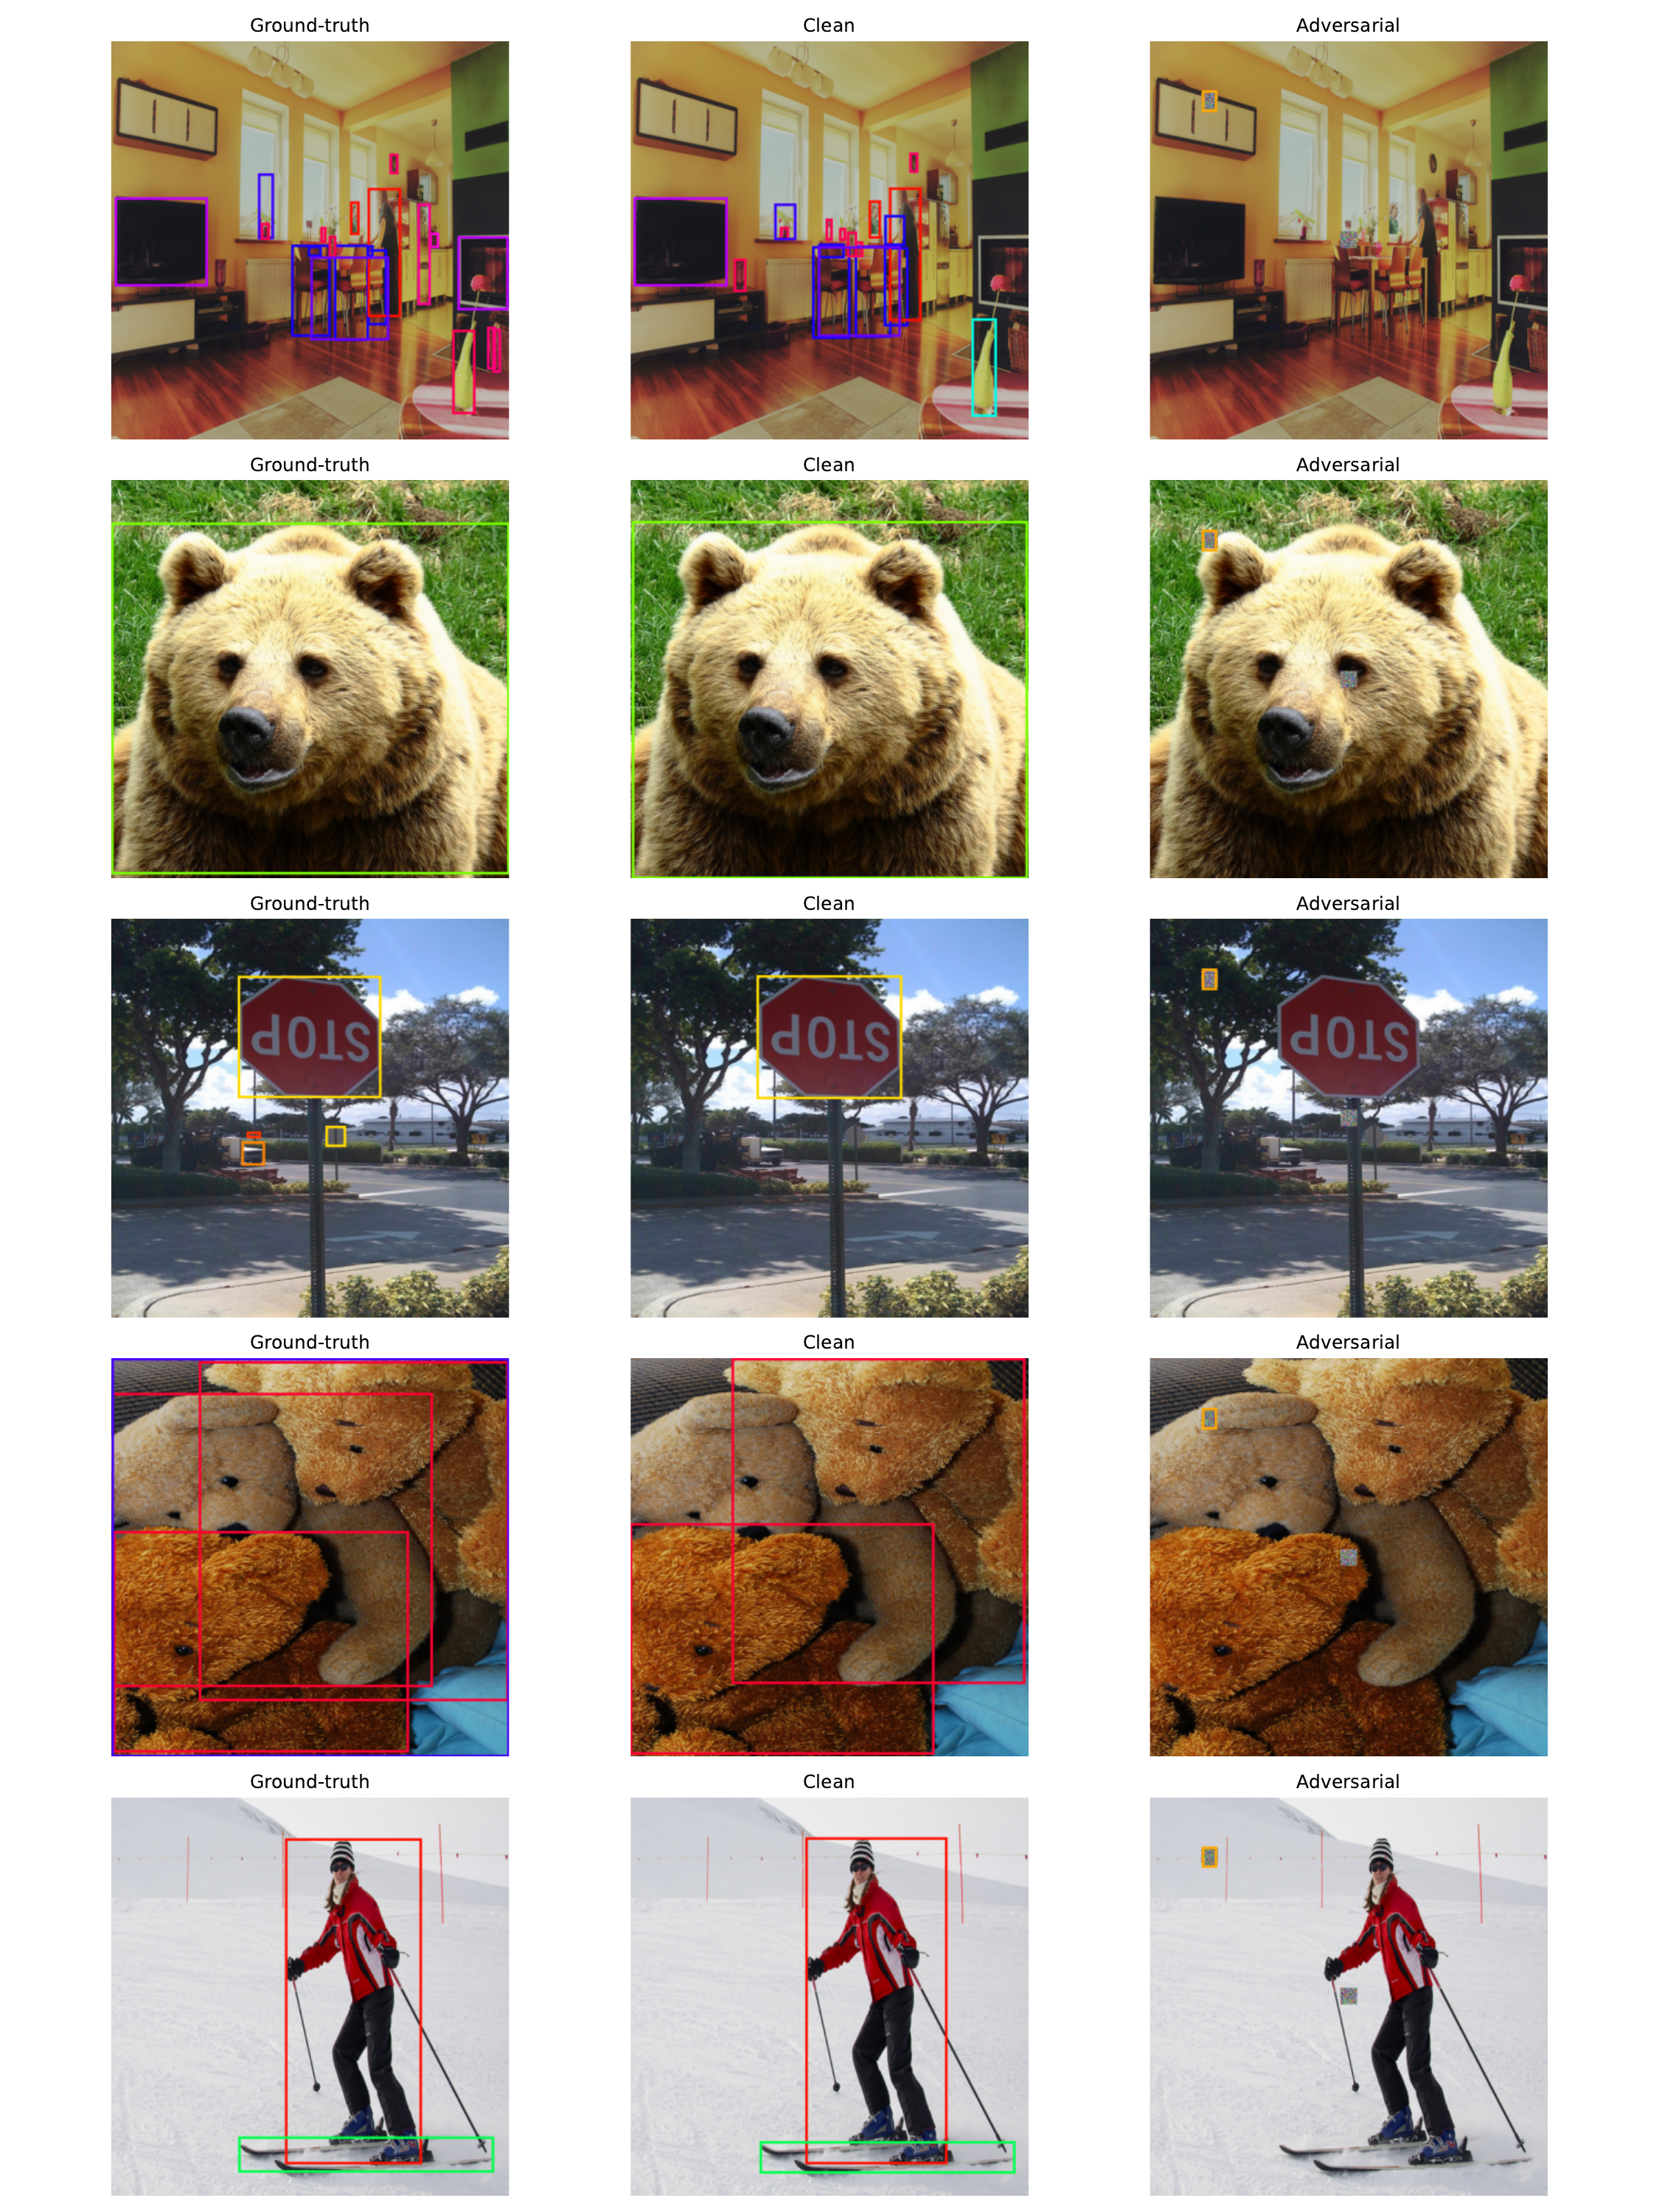}
        \caption{Bounding box comparison among ground-truth, clean images, and adversarial images in CP attack.}
        \label{fig:bbox_CP}
    \end{minipage}
\end{figure*}

\subsection{Change in attention heatmaps and pointer heatmaps}
In Fig. \ref{fig:heatmap_SP} and \ref{fig:heatmap_CP}, we illustrate the evolving snapshots of the pointer and attention redirected towards the target patch as epochs increase in the case of SP and CP attacks.

\begin{figure*}[h]
    \centering
    \begin{minipage}{\textwidth}
        \includegraphics[width=\linewidth]{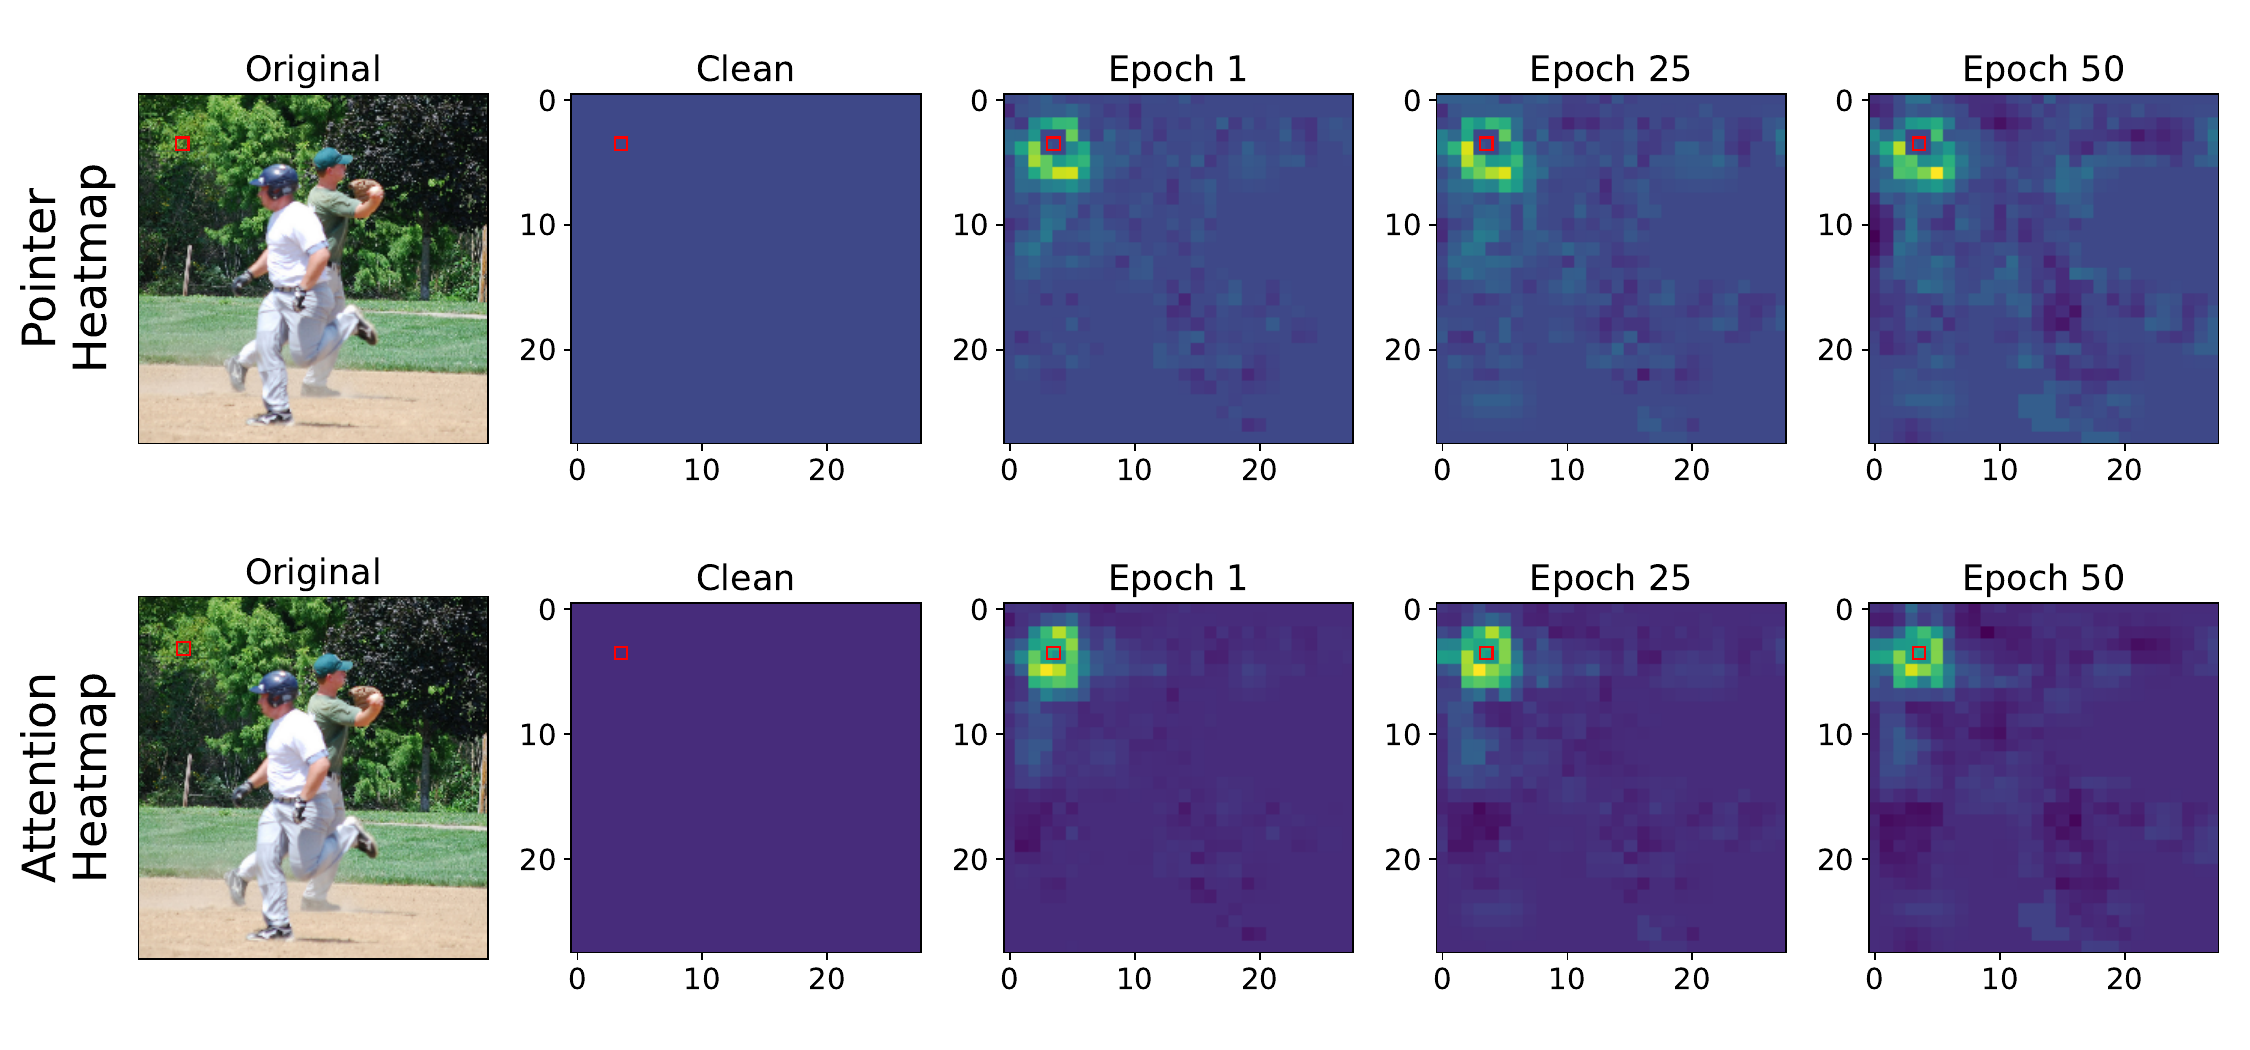}
    \end{minipage}
        \begin{minipage}{\textwidth}
        \includegraphics[width=\linewidth]{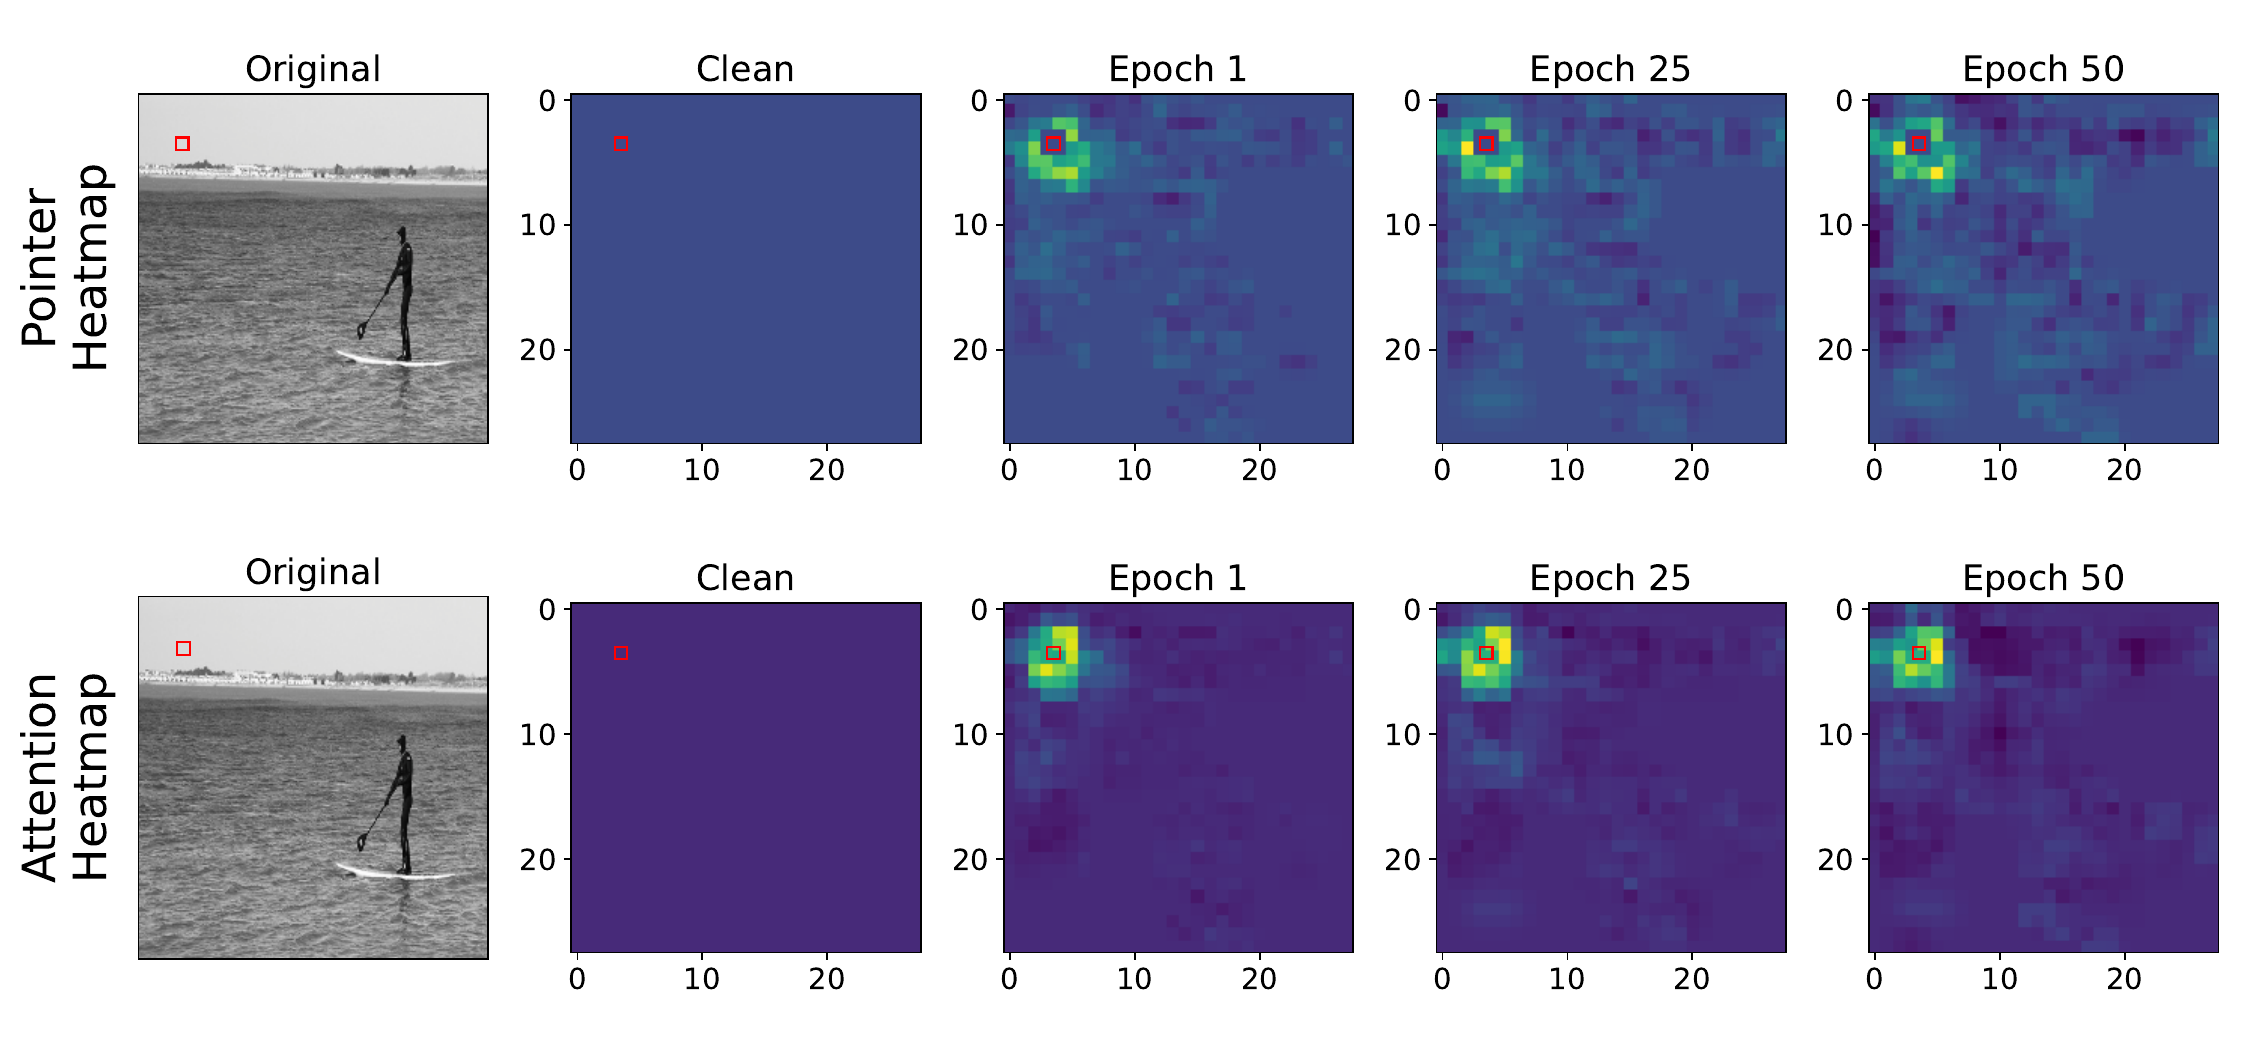}
    \end{minipage}
    \caption{Pointer and attention redirect toward the target patch for SP attack}
    \label{fig:heatmap_SP}
\end{figure*}

\begin{figure*}[h]
    \centering
    \begin{minipage}{\textwidth}
        \includegraphics[width=\linewidth]{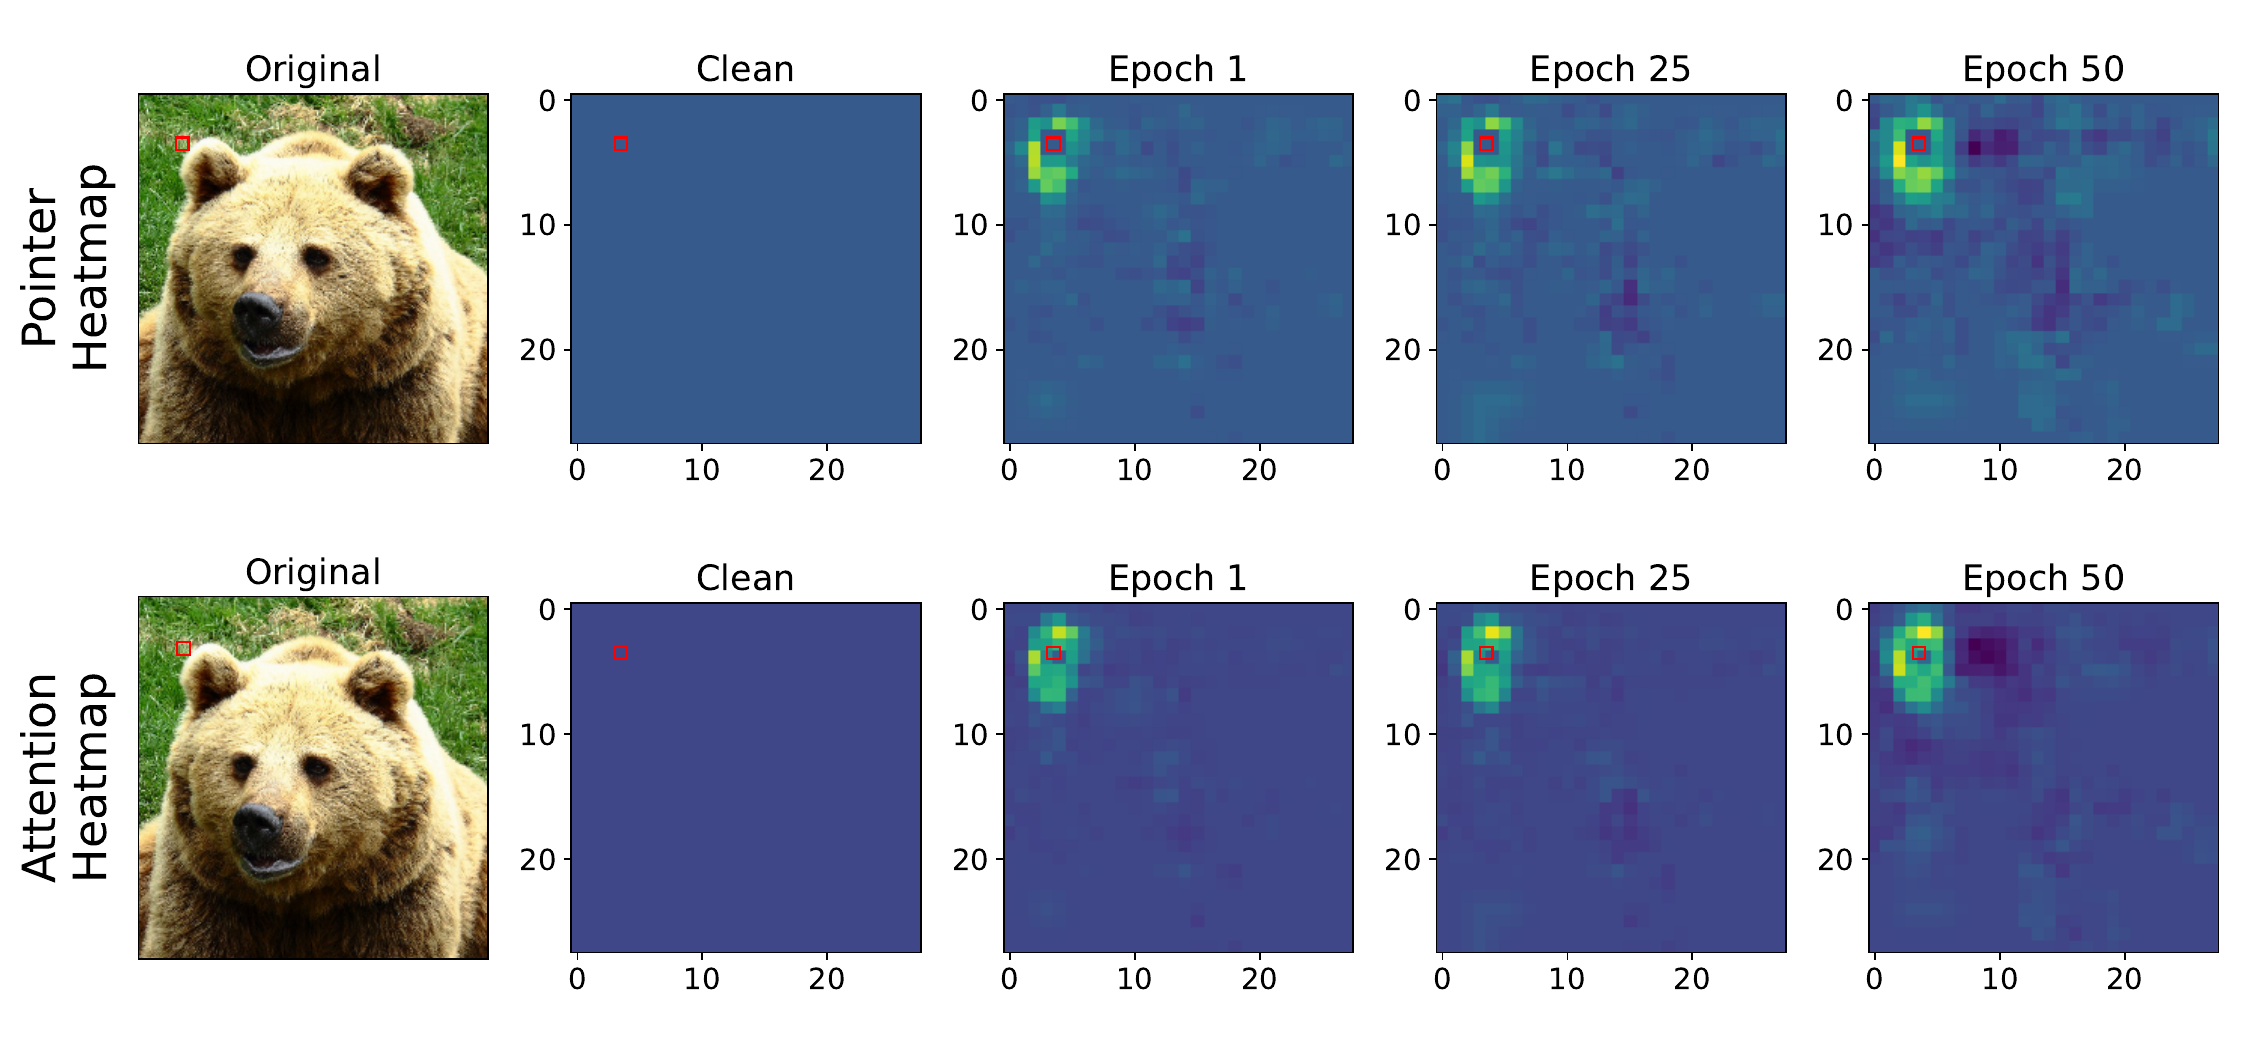}
    \end{minipage}
        \begin{minipage}{\textwidth}
        \includegraphics[width=\linewidth]{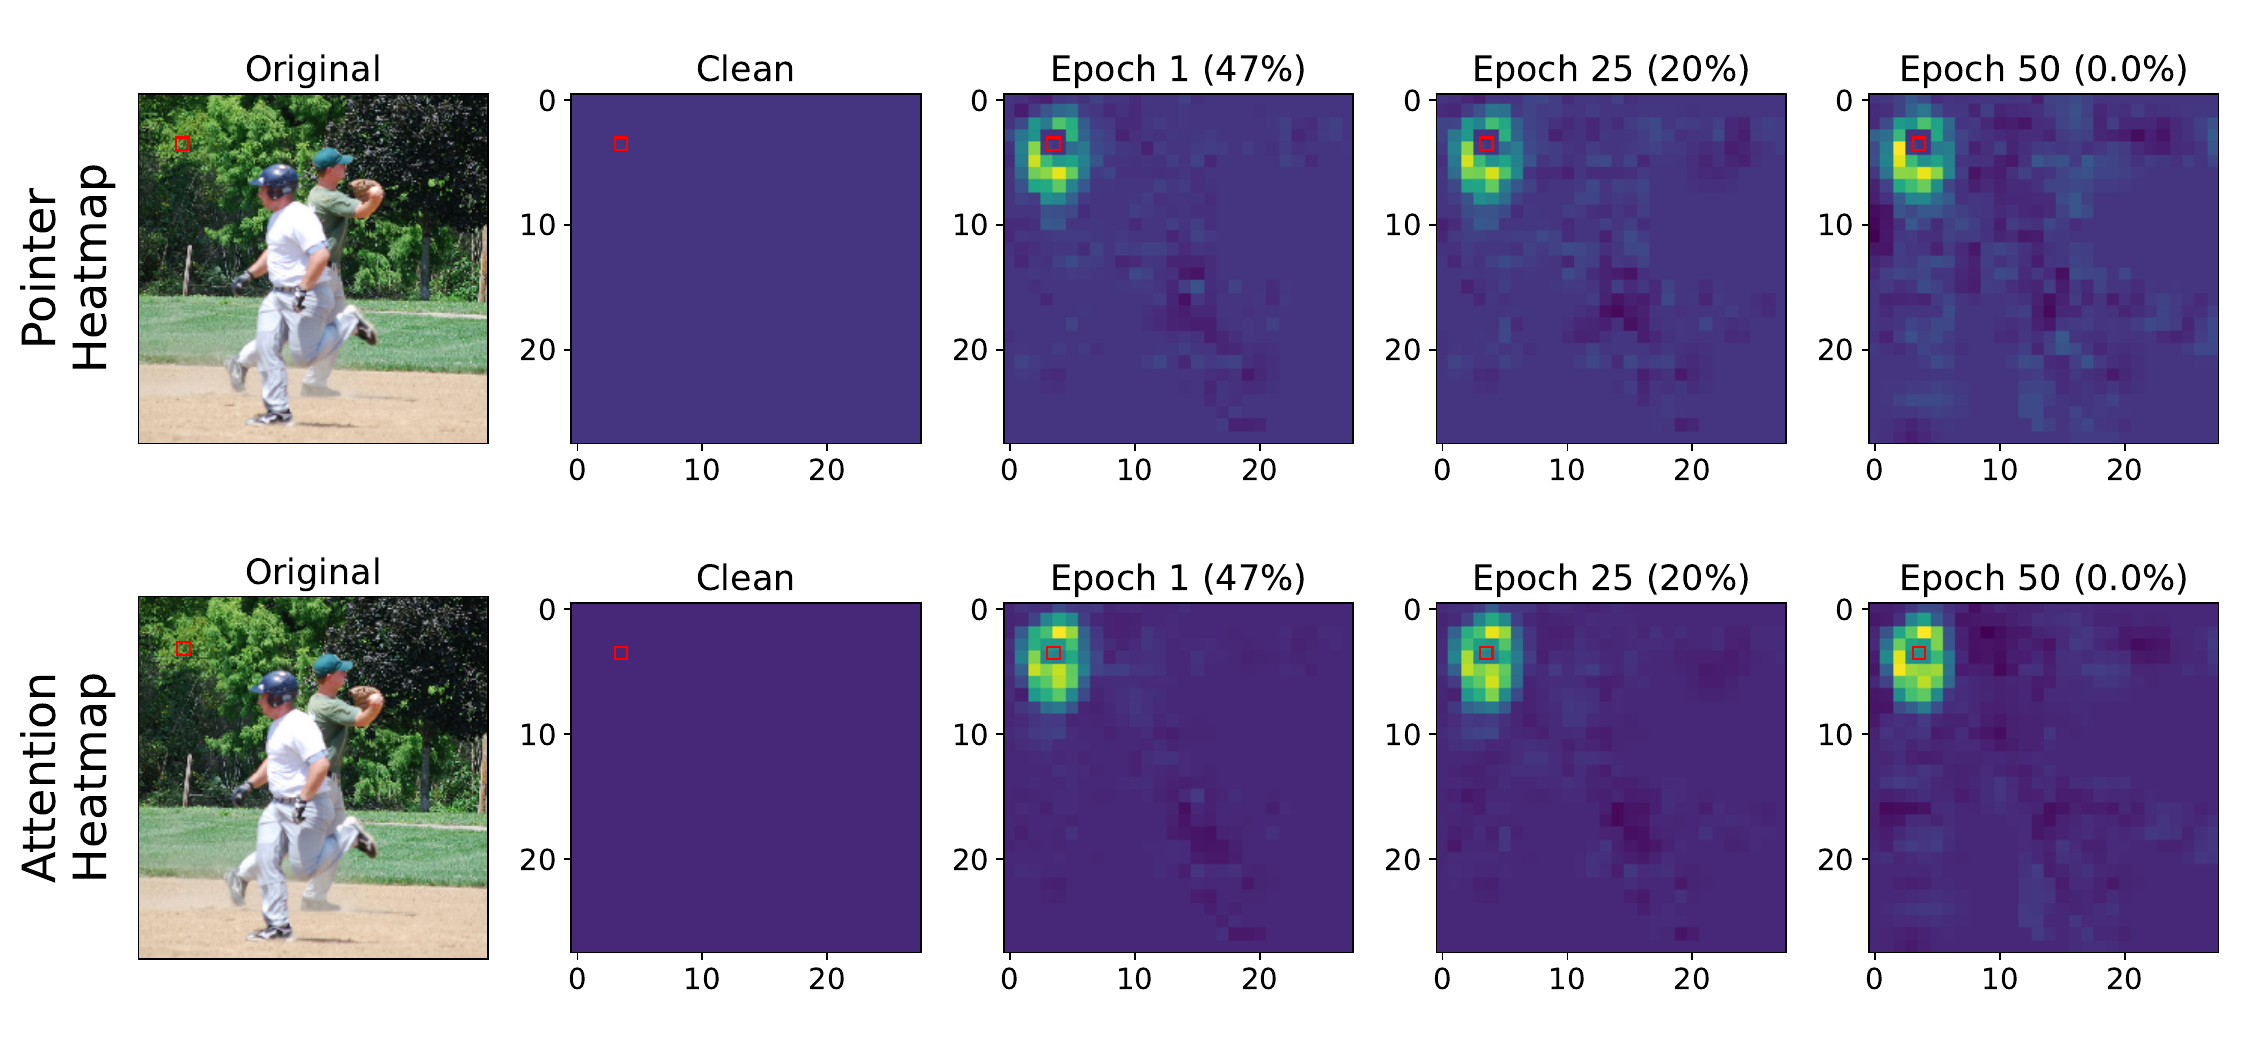}
    \end{minipage}
    \caption{Pointer and attention redirect toward the target patch for CP attack}
    \label{fig:heatmap_CP}
\end{figure*}

\section{Illustration of attack on MvDeTr}
In Fig. \ref{fig:IP}, \ref{fig:OP}, \ref{fig:CP}, \ref{fig:SP} we also show the illustration of IP, OP, CP, SP attacks on Wildtrack dataset with 7 camera views and MvDeTr model. For each attack we show the objects detection results in each view. Note that, the attacks will not completely get rid of the bounding-boxes, but rather adversarially attack the locations and sizes of the bounding boxes. In each view, we see a lot less bounding boxes, also the bounding boxes that are present are also off. In the next figures (Fig. \ref{fig:hclean}, \ref{fig:hgt}, \ref{fig:hip}, \ref{fig:hop}, \ref{fig:hsp}, \ref{fig:hcp}) we also show the heatmap of the world plane, we see that for SP and CP attack the worldmaps are entirely different. World heatmap indicate where objects are present on the ground plane.

\begin{figure*}[t] % Use the star (*) to span both columns
    \centering
    \begin{minipage}{0.7\textwidth}
        \includegraphics[width=\linewidth]{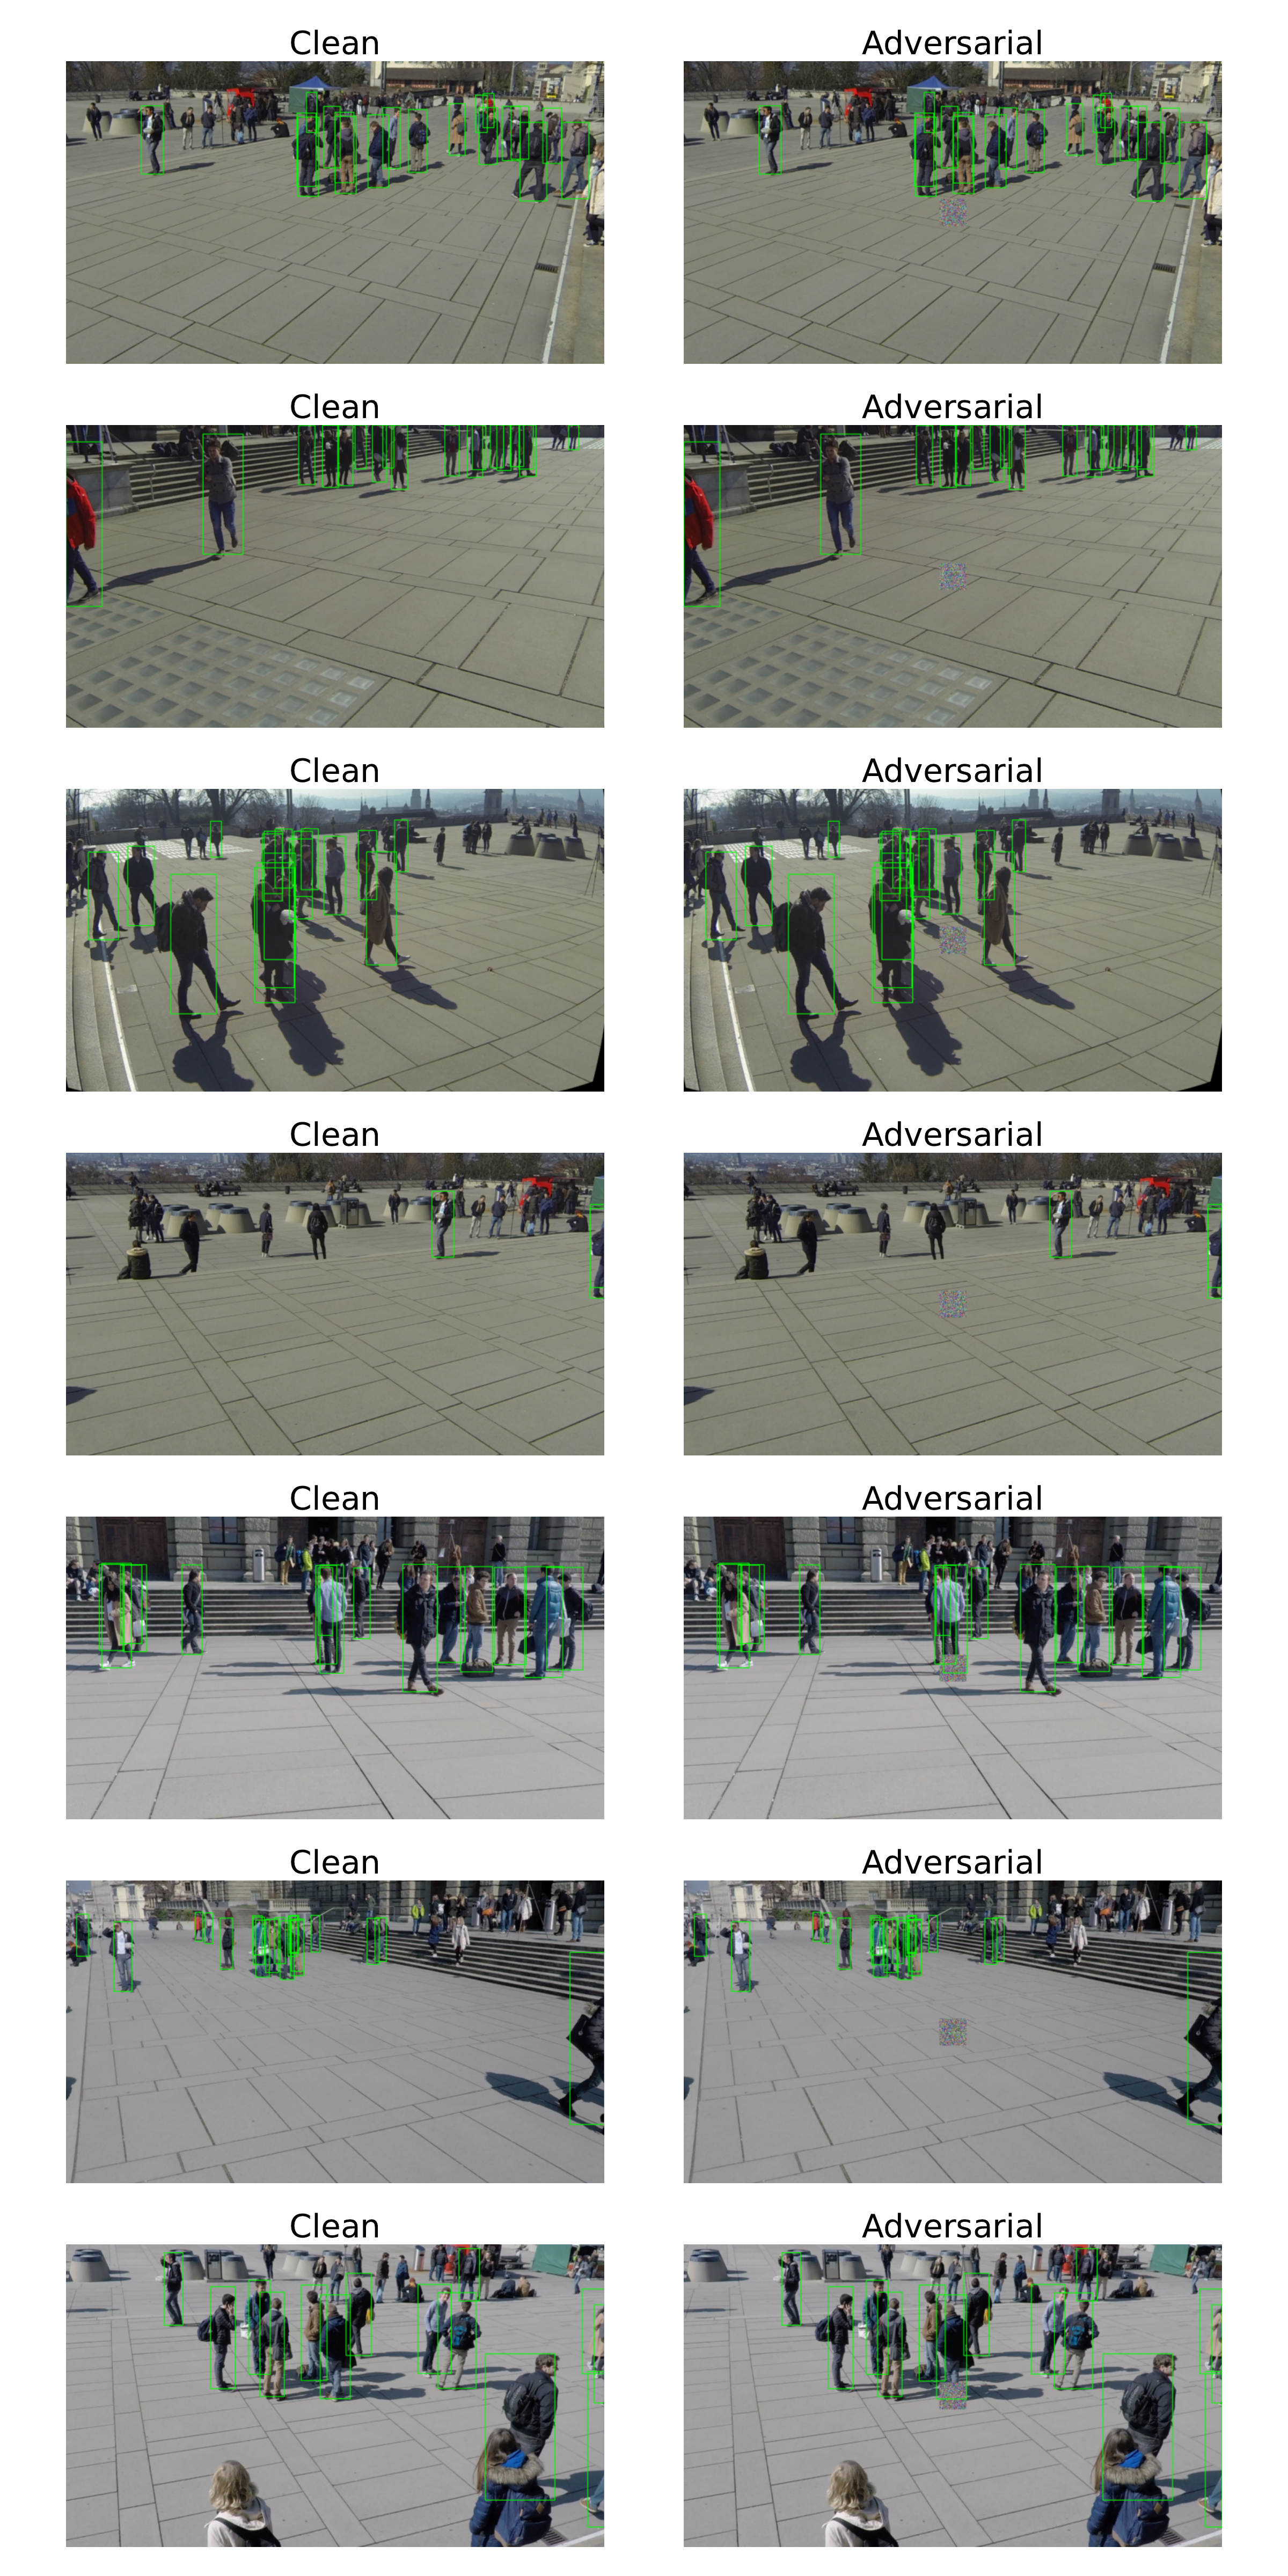}
        \caption{Bounding box comparison among 7 cameras in clean and adversarial in IP attack.}
        \label{fig:IP}
    \end{minipage}
\end{figure*}

\begin{figure*}[t] % Use the star (*) to span both columns
    \centering
    \begin{minipage}{0.7\textwidth}
        \includegraphics[width=\linewidth]{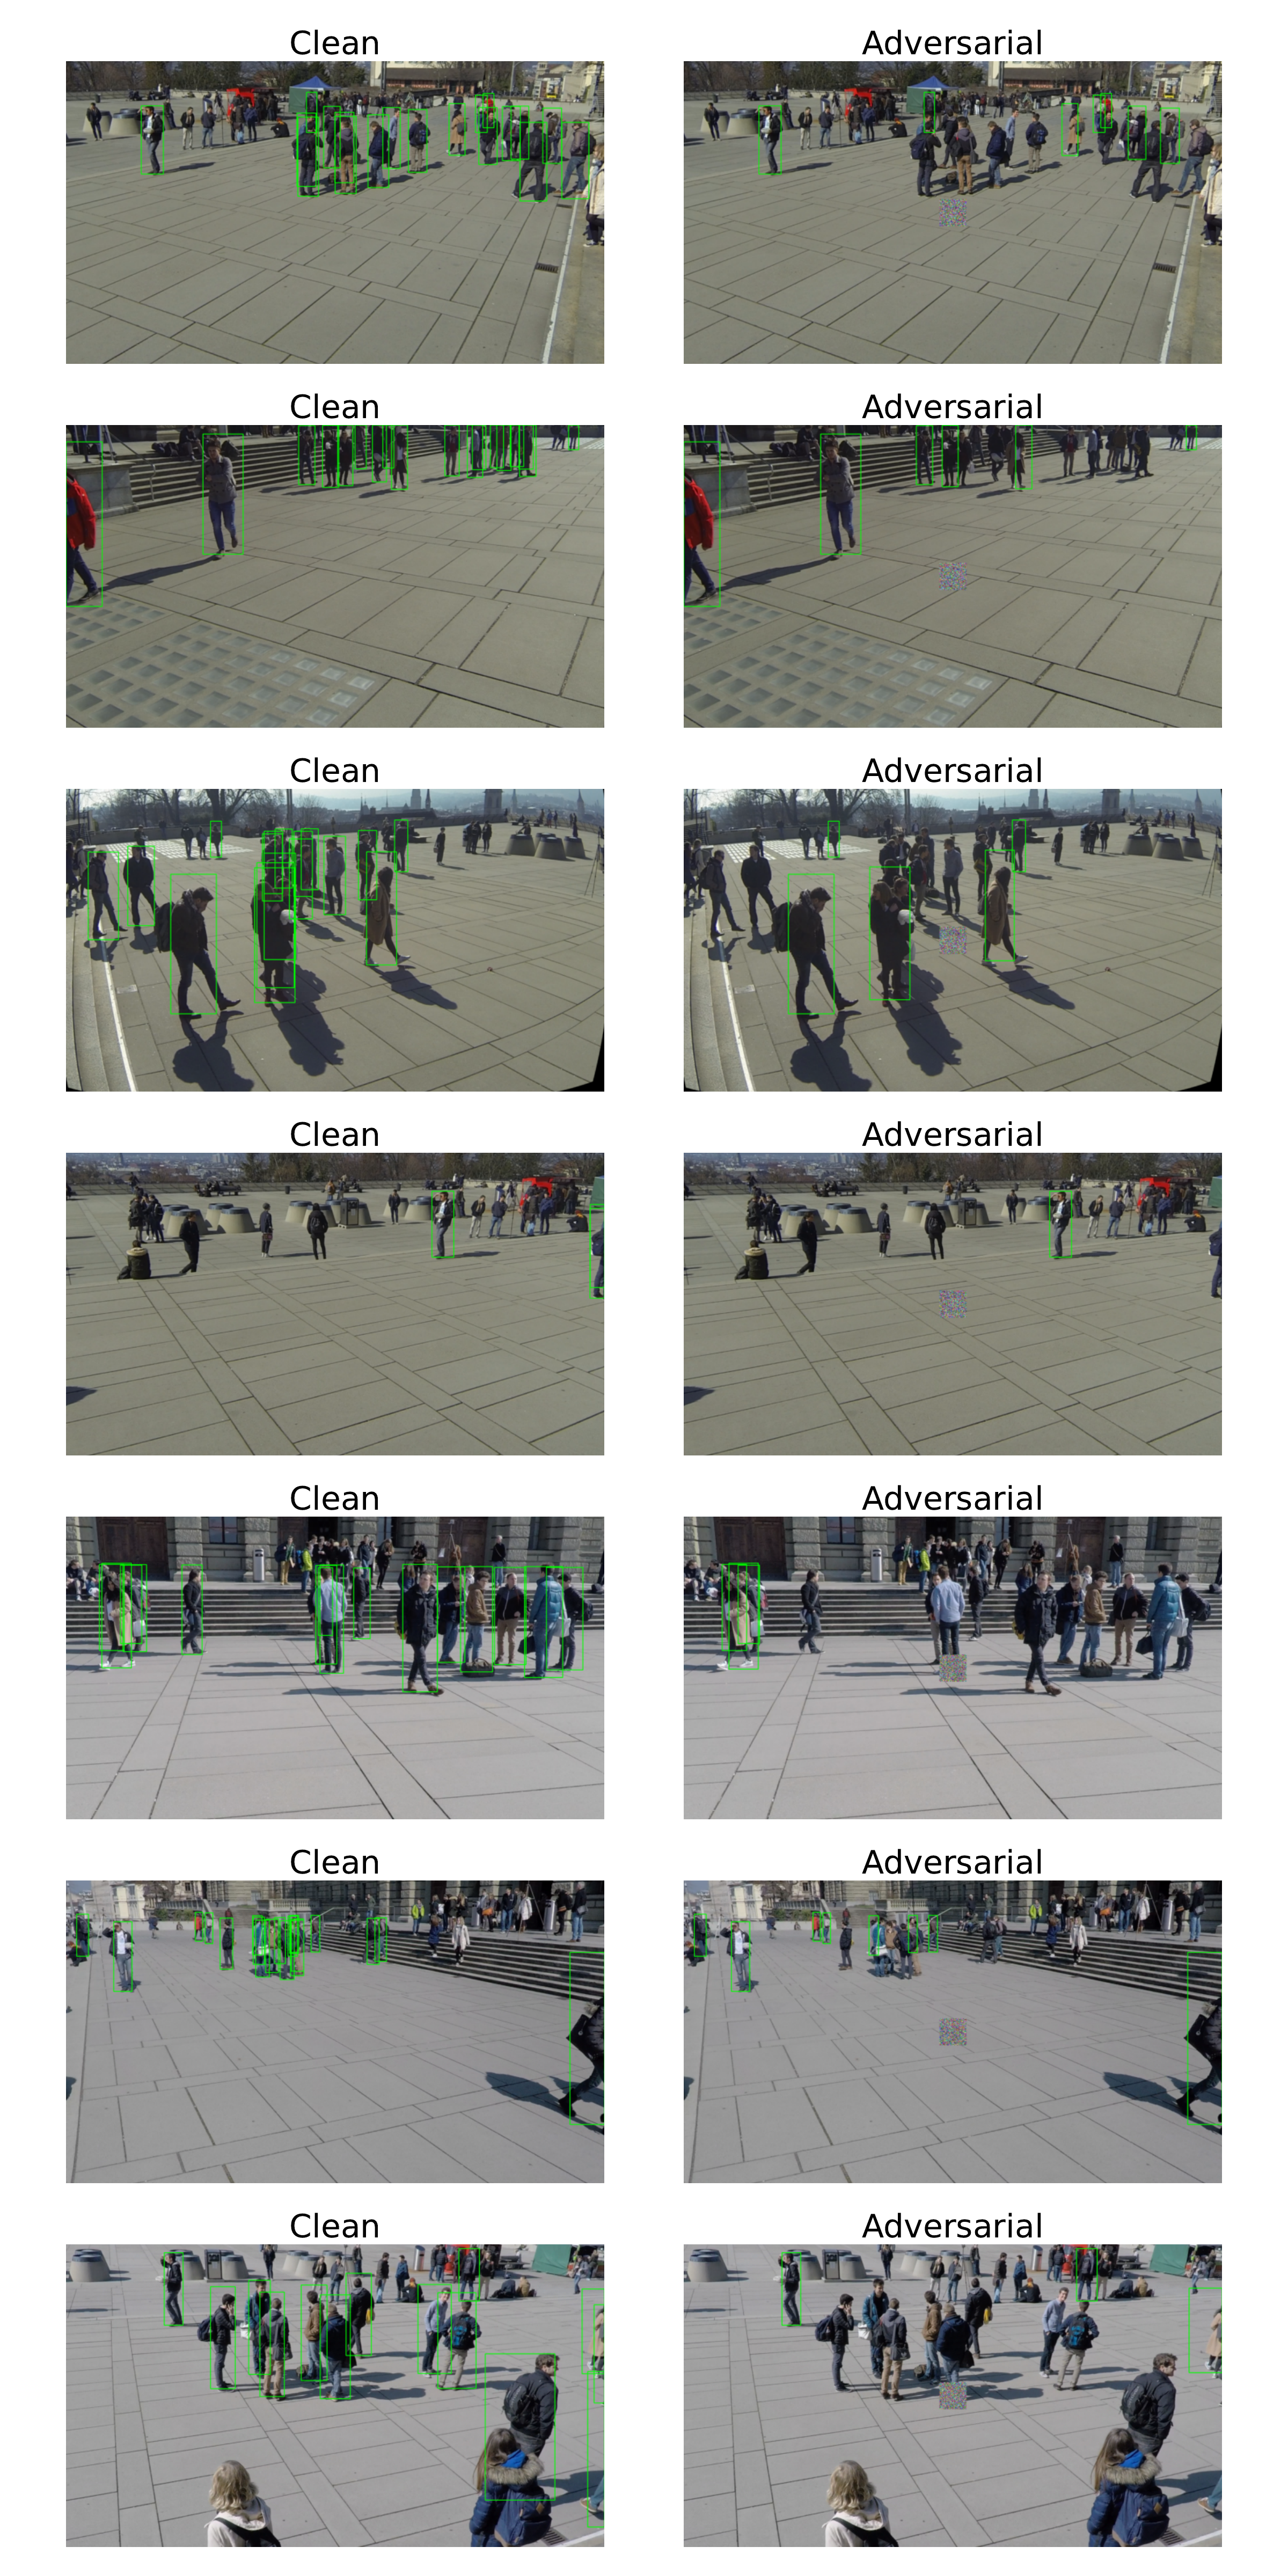}
        \caption{BBounding box comparison among 7 cameras in  clean and adversarial in OP attack.}
        \label{fig:OP}
    \end{minipage}
\end{figure*}

\begin{figure*}[t] % Use the star (*) to span both columns
    \centering
    \begin{minipage}{0.7\textwidth}
        \includegraphics[width=\linewidth]{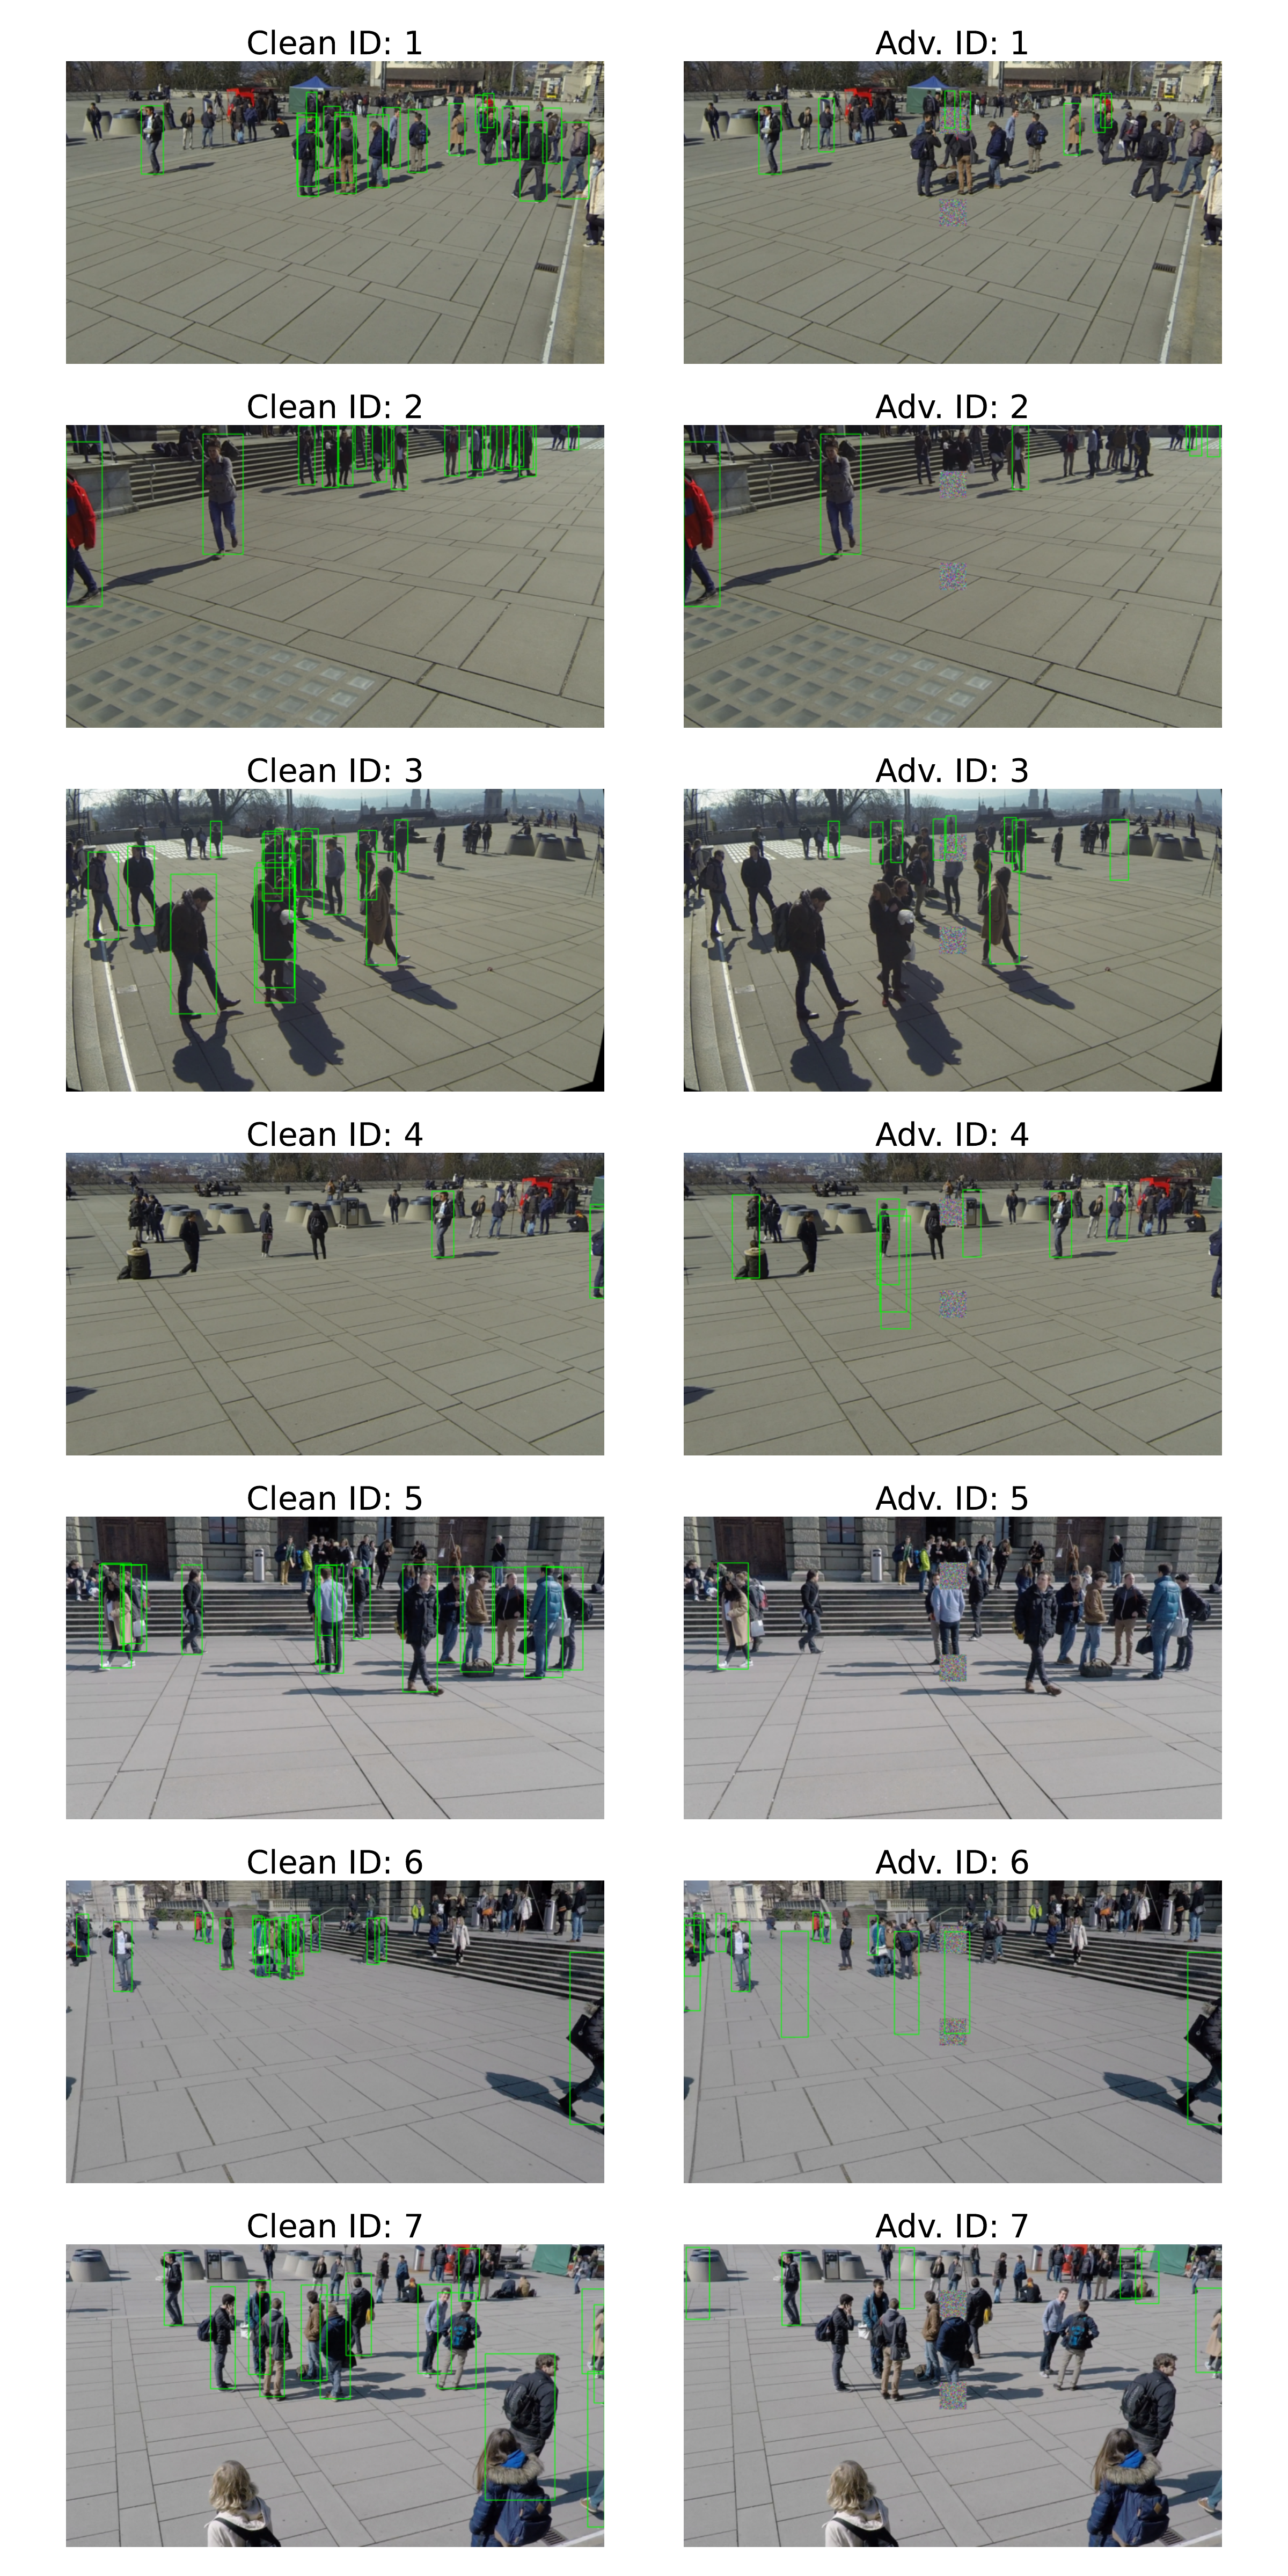}
        \caption{Bounding box comparison among 7 cameras in  clean and adversarial in CP attack.}
        \label{fig:CP}
    \end{minipage}
\end{figure*}

\begin{figure*}[t] % Use the star (*) to span both columns
    \centering
    \begin{minipage}{0.7\textwidth}
        \includegraphics[width=\linewidth]{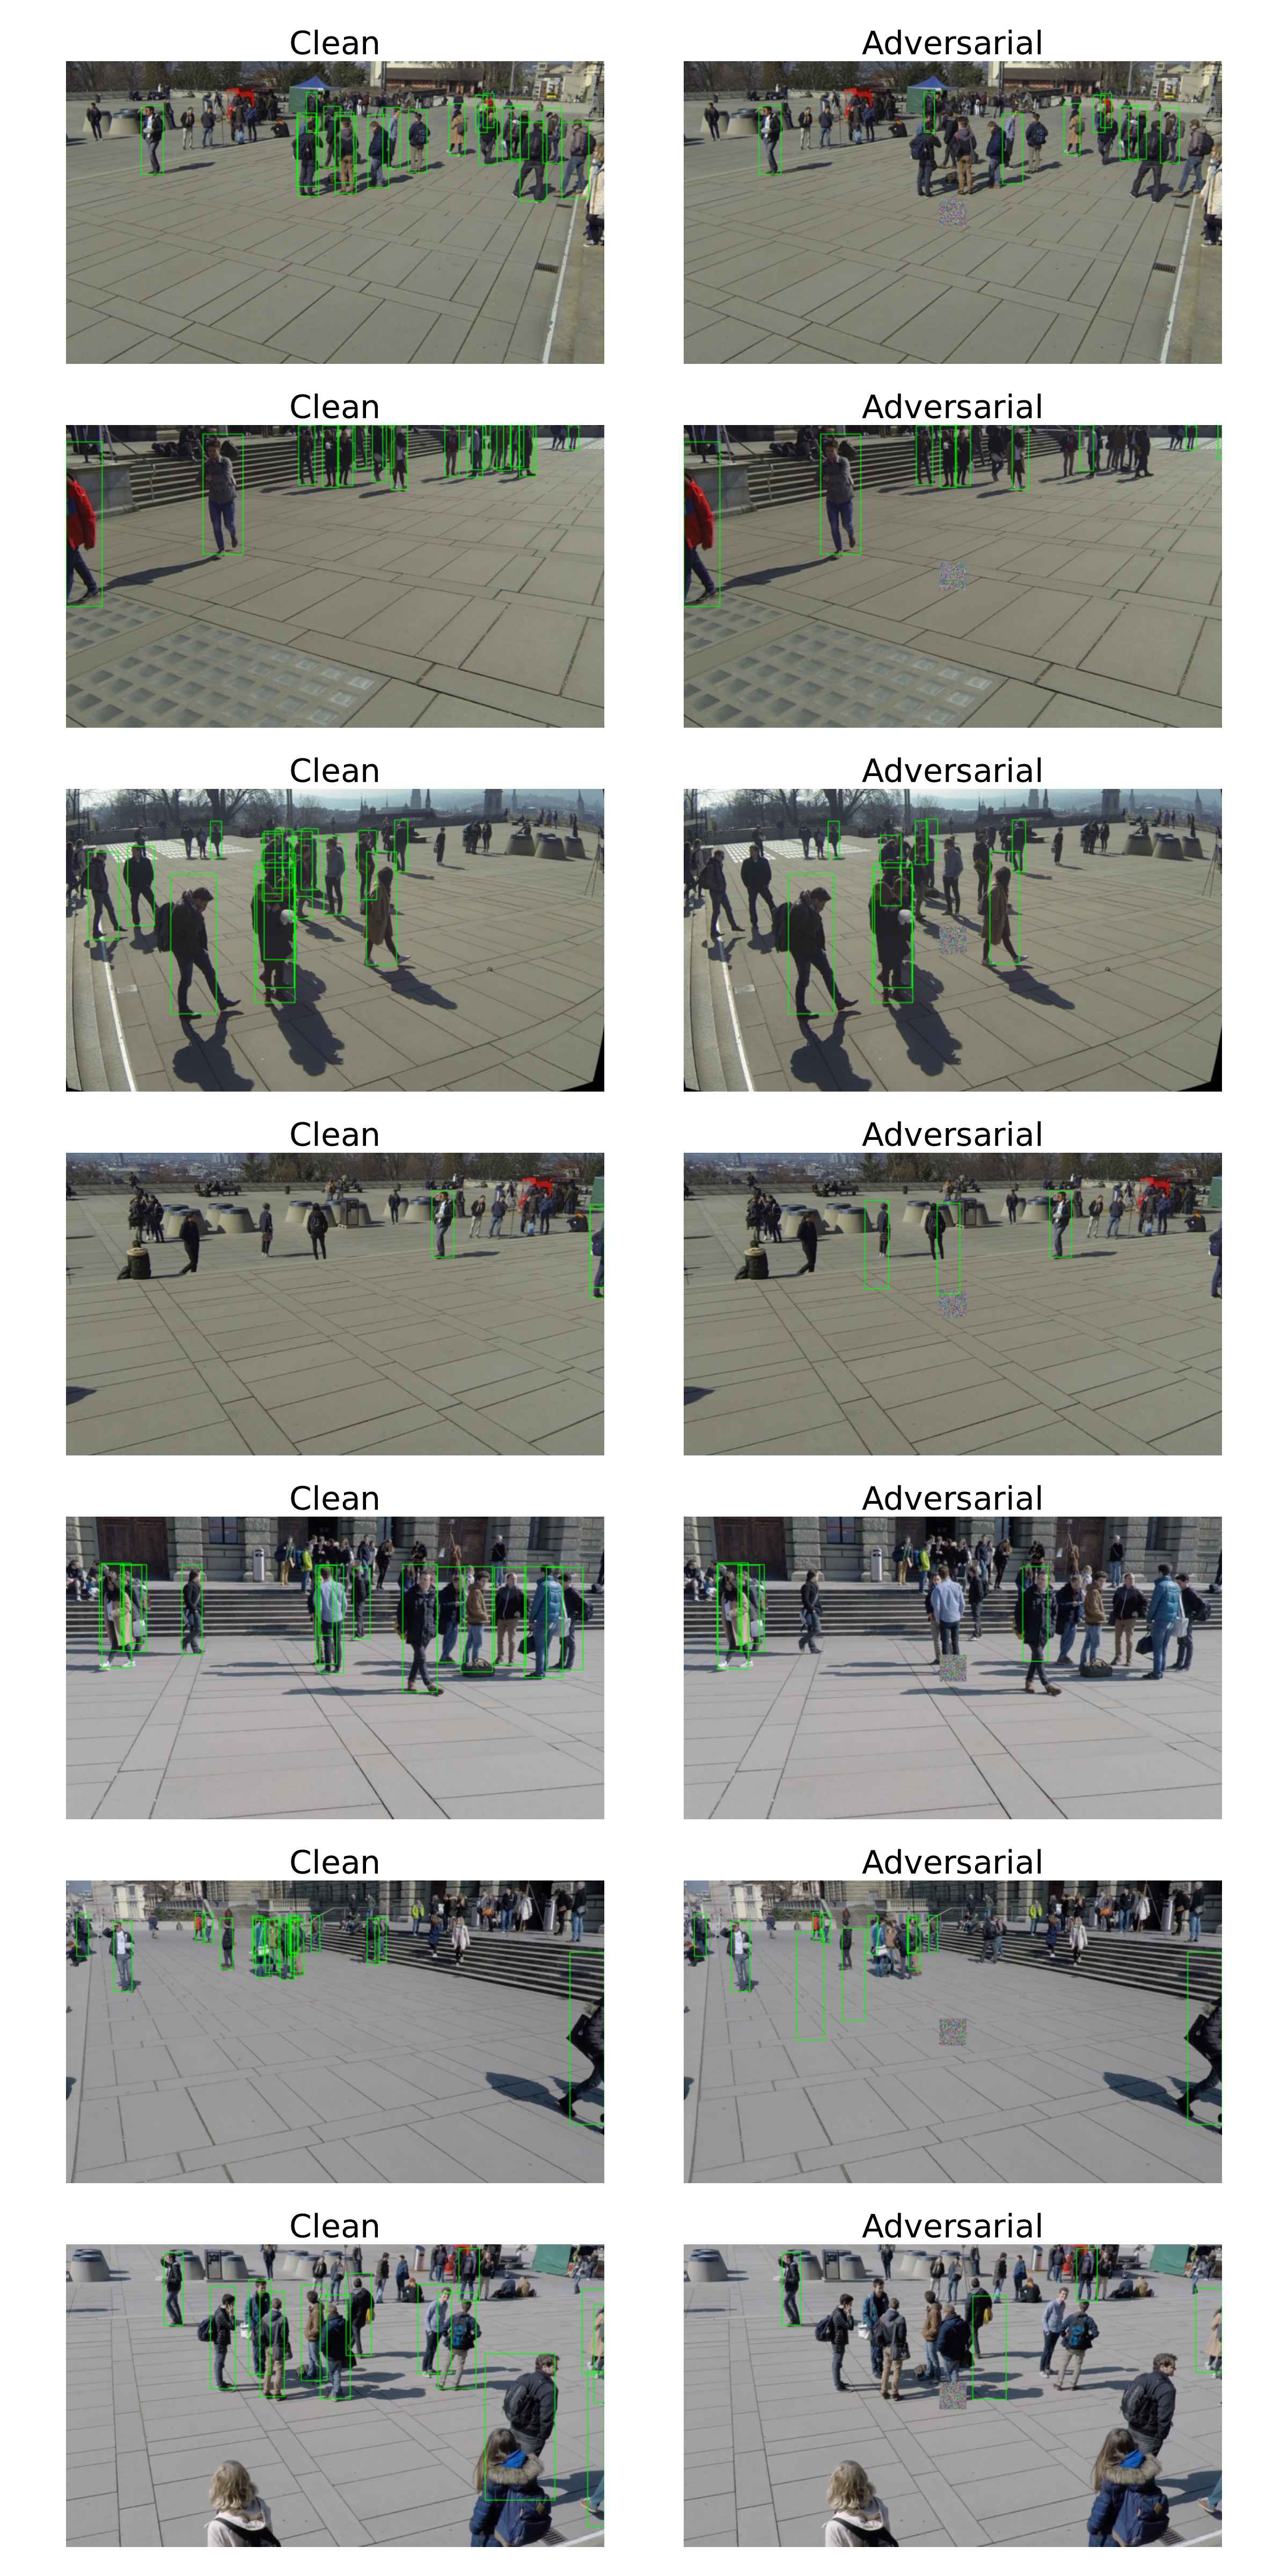}
        \caption{Bounding box comparison among 7 cameras in  clean and adversarial in SP attack.}
        \label{fig:SP}
    \end{minipage}
\end{figure*}

\clearpage

\begin{figure}[h]
    \centering
    \includegraphics[width=\linewidth]{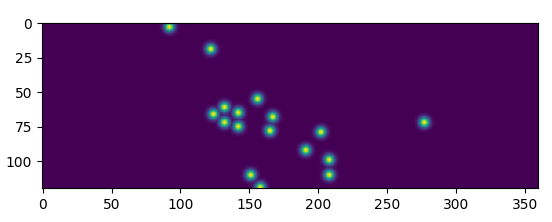}
    \caption{Ground-truth world hmap}
    \label{fig:hgt}
\end{figure}

\begin{figure}[h]
    \centering
    \includegraphics[width=\linewidth]{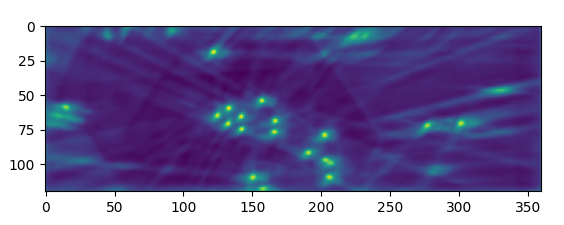}
    \caption{Clean world hmap}
    \label{fig:hclean}
\end{figure}

\begin{figure}[h]
    \centering
    \includegraphics[width=\linewidth]{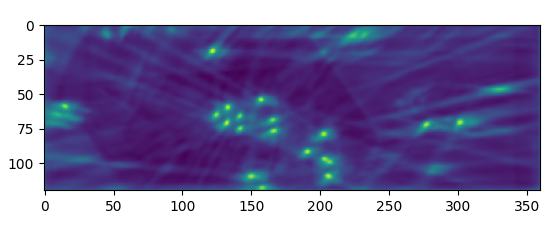}
    \caption{IP world hmap}
    \label{fig:hip}
\end{figure}

\begin{figure}[h]
    \centering
    \includegraphics[width=\linewidth]{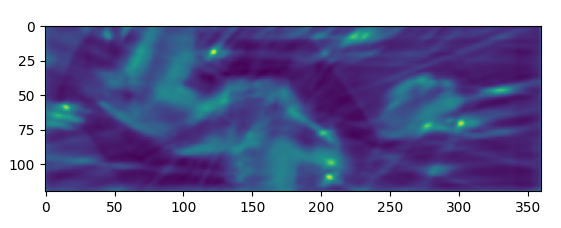}
    \caption{OP world hmap}
    \label{fig:hop}
\end{figure}

\begin{figure}[h]
    \centering
    \includegraphics[width=\linewidth]{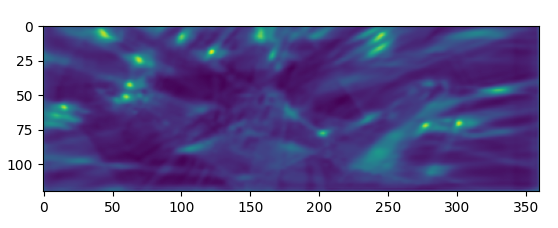}
    \caption{CP world hmap}
    \label{fig:hcp}
\end{figure}

\begin{figure}[h]
    \centering
    \includegraphics[width=\linewidth]{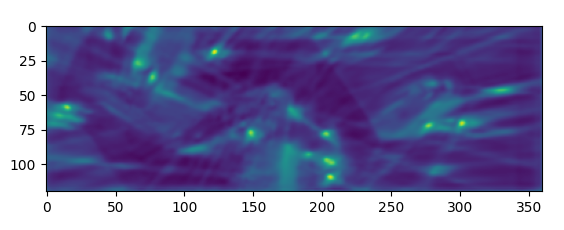}
    \caption{SP world hmap}
    \label{fig:hsp}
\end{figure}

\clearpage
\section{Training curves}
\subsection{Training curves of all the attack}
In Fig. \ref{fig:training-curve} we show the training curve of all attacks on DeTr. We observe that the attacks (SP and CP) associated with traditional adversarial patches based on model loss converge faster than the attacks that are not (IP and OP). In these experiments we used a 32x32 sized patch for single patch attacks (e.g., IP, OP, SP, Att) and two 23x23 patch for multi patch attacks (e.g., CP).

\begin{figure}[h]
    \centering
    \includegraphics[width=\linewidth]{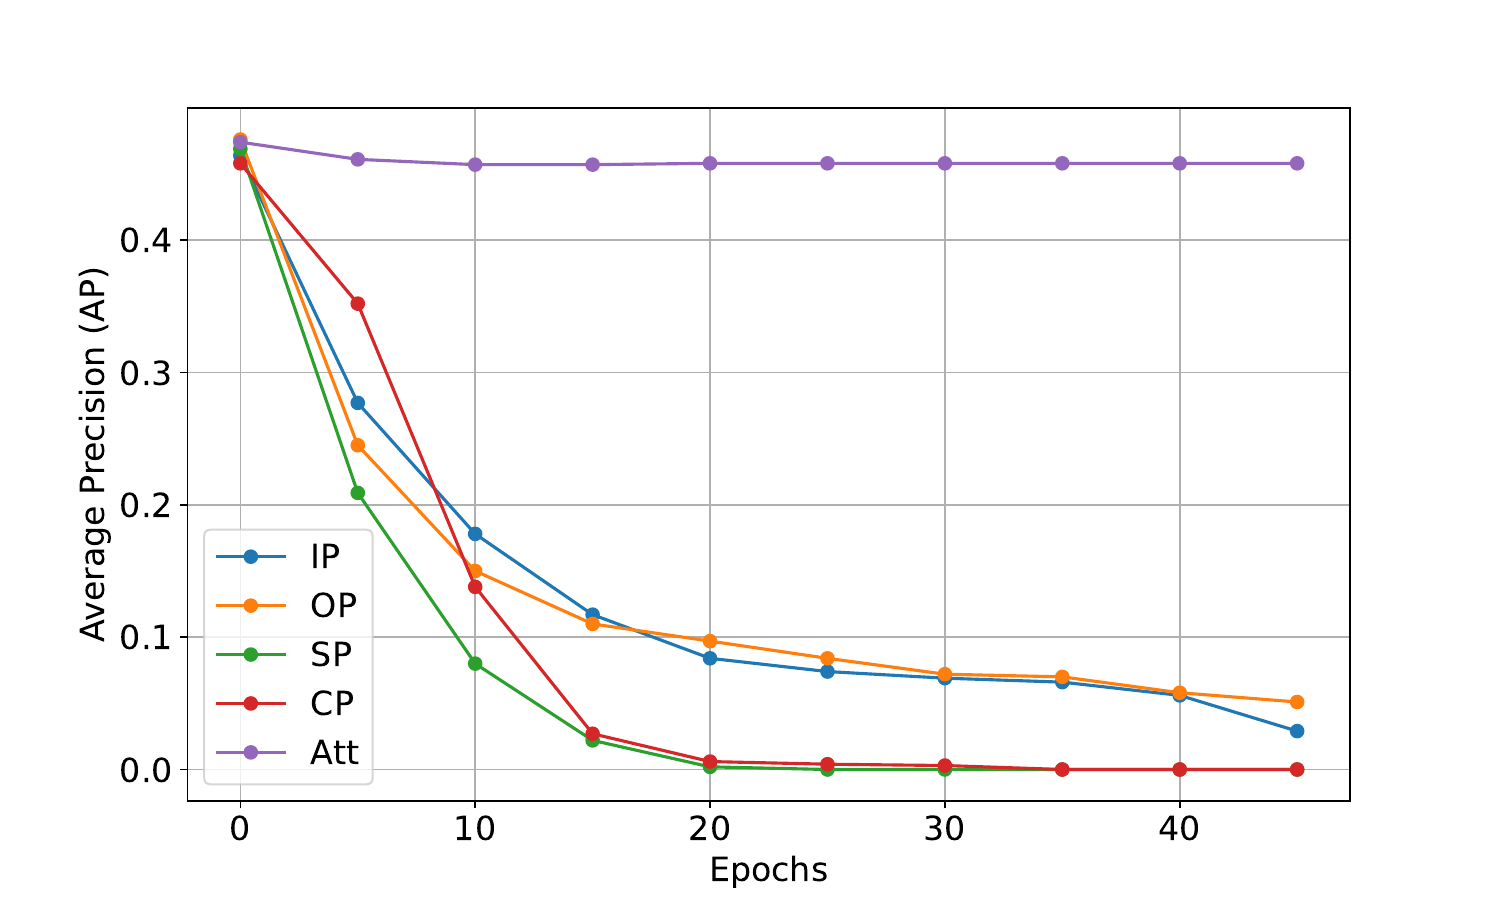}
    \caption{Training curve of all the attacks}
    \label{fig:training-curve}
\end{figure}

\subsection{Training curves for increasing patch sizes}
For this experiment, we choose the CP attack on DeTr as it has both source and target patches, and show how varying their size affect the training curve. In Fig. \ref{fig:training-curve-source-size} we see that with increasing source sizes the training converges faster. Moreover, as depicted in Fig. \ref{fig:training-curve-target-size}, it is observed that the training converges more rapidly with an increase in target size. Notably, patches of size 12x12, 24x24, and 36x36 cluster together with comparable progress, whereas the 48x48 patch converges at a much faster rate. For these experiments, we only use one source patch and one traget patch.

\begin{figure}[h]
    \centering
    \includegraphics[width=\linewidth]{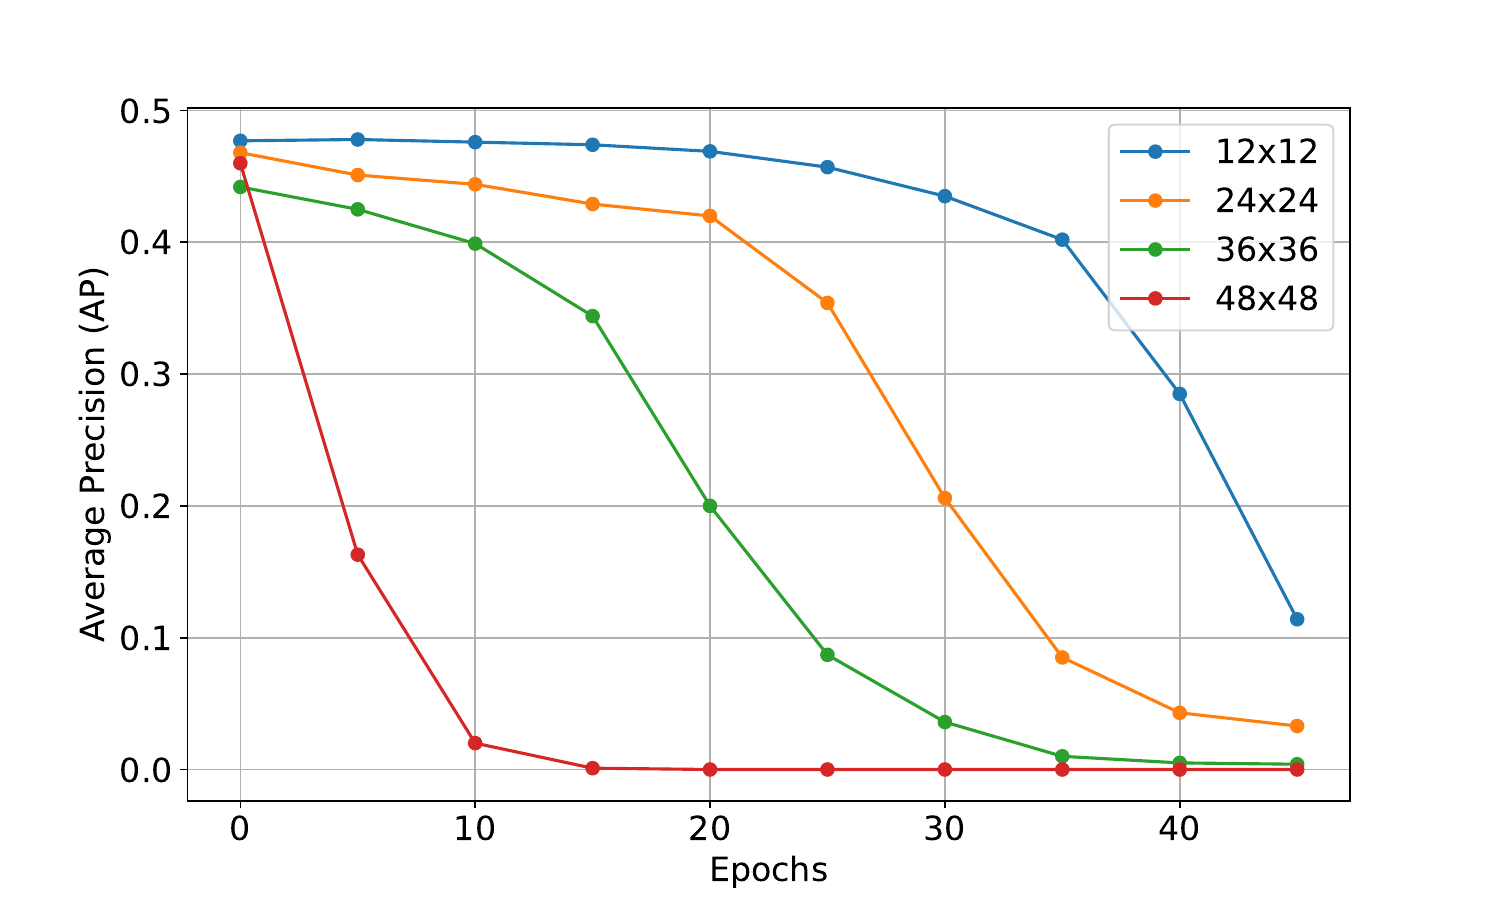}
    \caption{Training curve for increasing source sizes}
    \label{fig:training-curve-source-size}
\end{figure}

\begin{figure}[h]
    \centering
    \includegraphics[width=\linewidth]{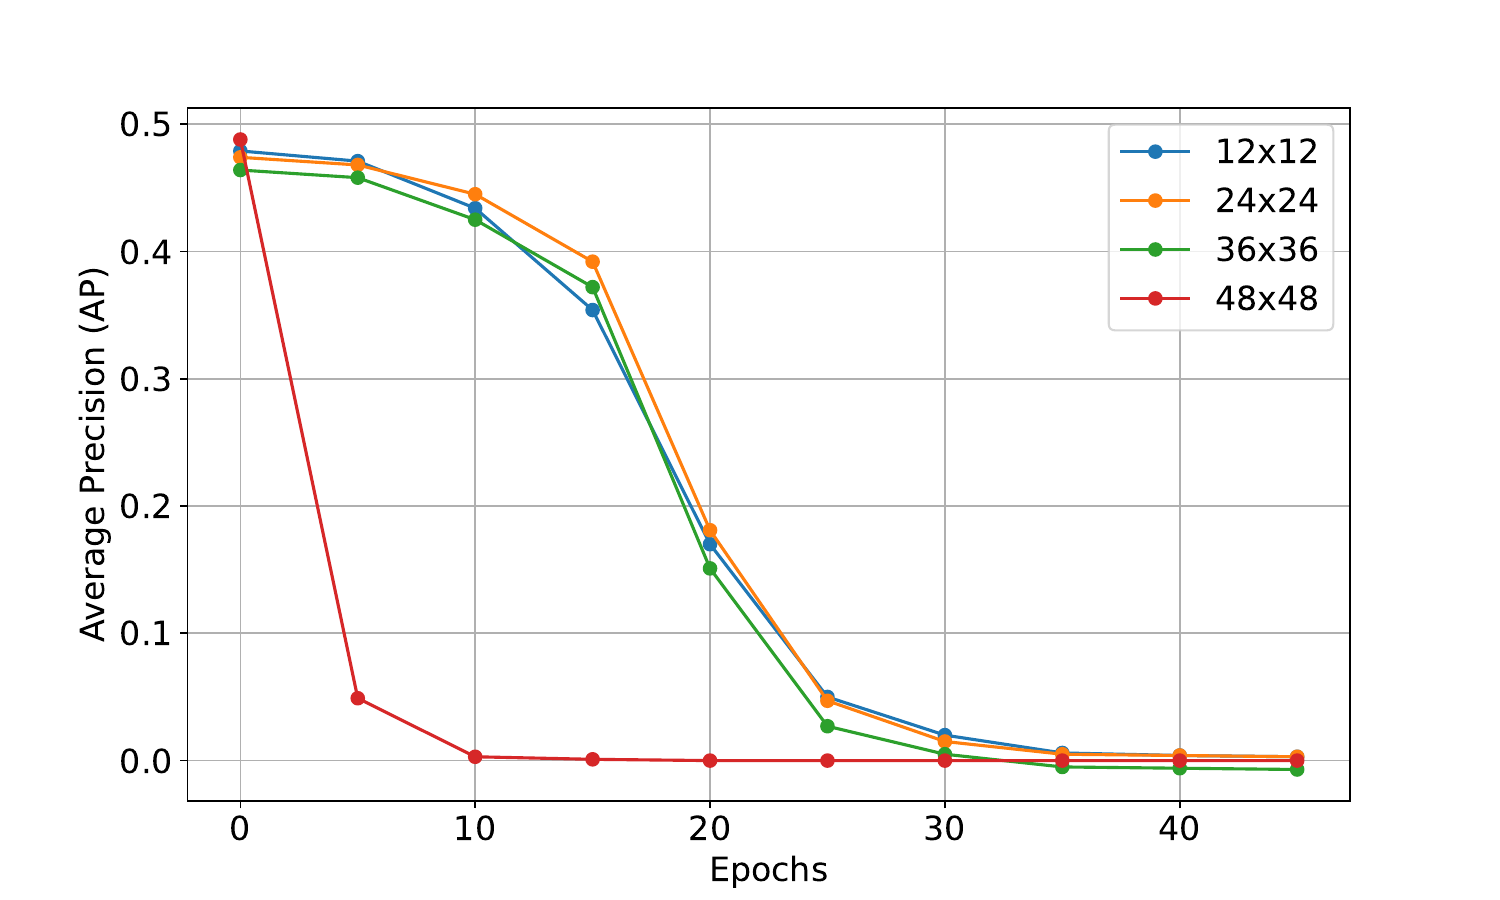}
    \caption{Training curve for increasing target sizes}
    \label{fig:training-curve-target-size}
\end{figure}

\subsection{Training curves for increasing patch counts}
For these experiments, we choose the CP attack on MVDeTr as CP has both source and target patches, and MVDeTr (4 patches in 7 views equals 28 patches in total) allows more patches than DeTr. In Fig. \ref{fig:training-curve-num-src} and \ref{fig:training-curve-num-tar} we see that with increasing number of source and target patches the attack converges faster. In this experiment, both source and target patches had a size of 32x32. To observe the effect of increasing source patch count, we uniformly increased the number of source patches in each view, while keeping a single target patch in each view. Similarly, to observe the effect of increasing target count, we uniformly increased the number of target patches in each view, while keeping a single source patch in each view.

\begin{figure}[h]
    \centering
    \includegraphics[width=\linewidth]{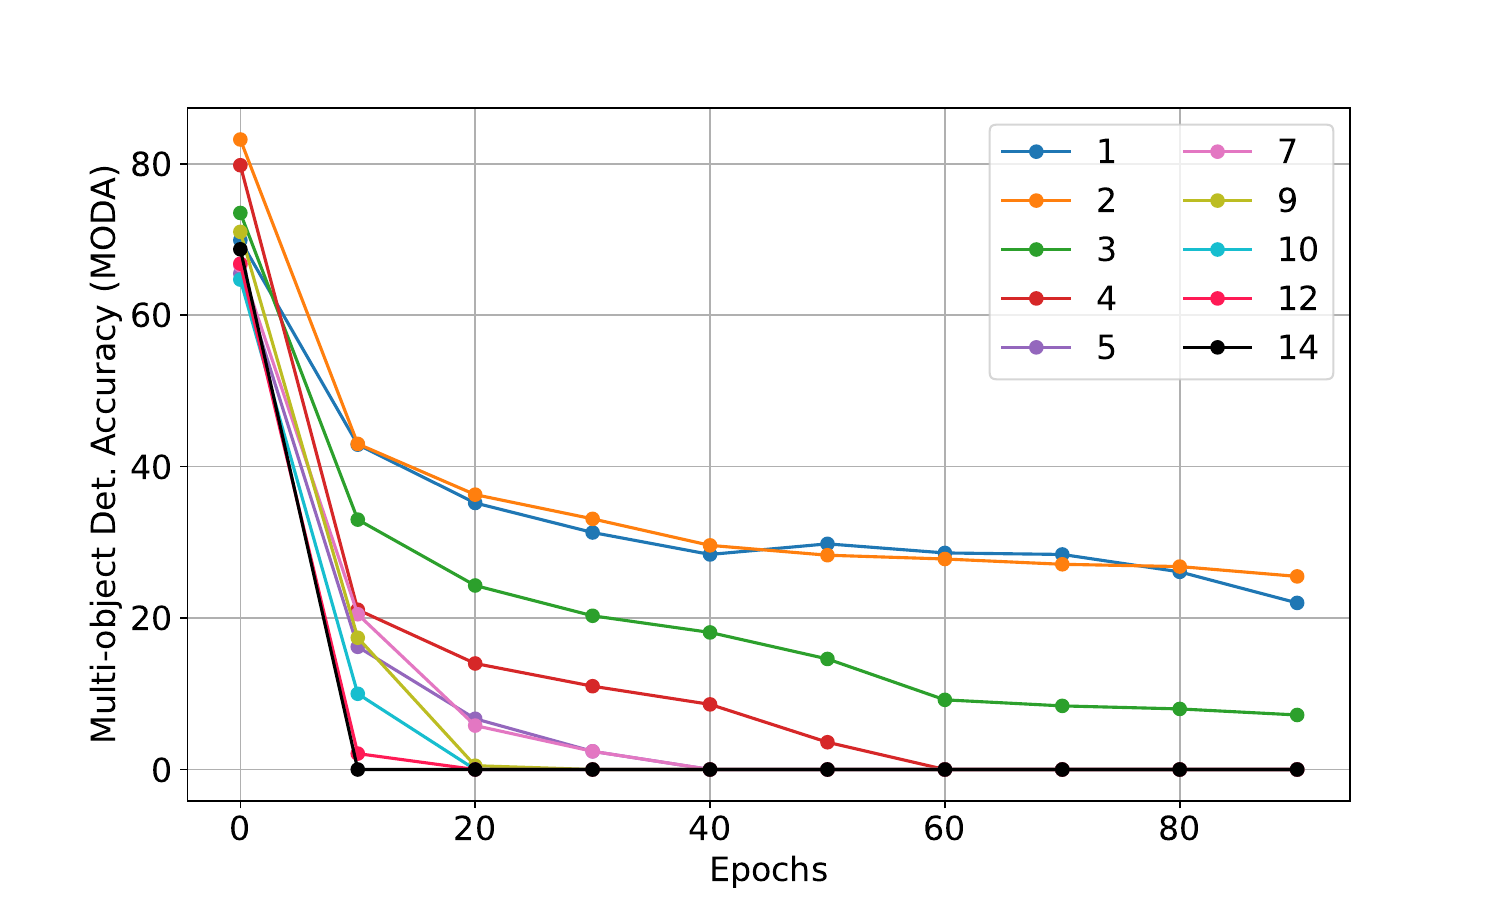}
    \caption{Training curve for increasing number of source patches}
    \label{fig:training-curve-num-src}
\end{figure}

\begin{figure}[h]
    \centering
    \includegraphics[width=\linewidth]{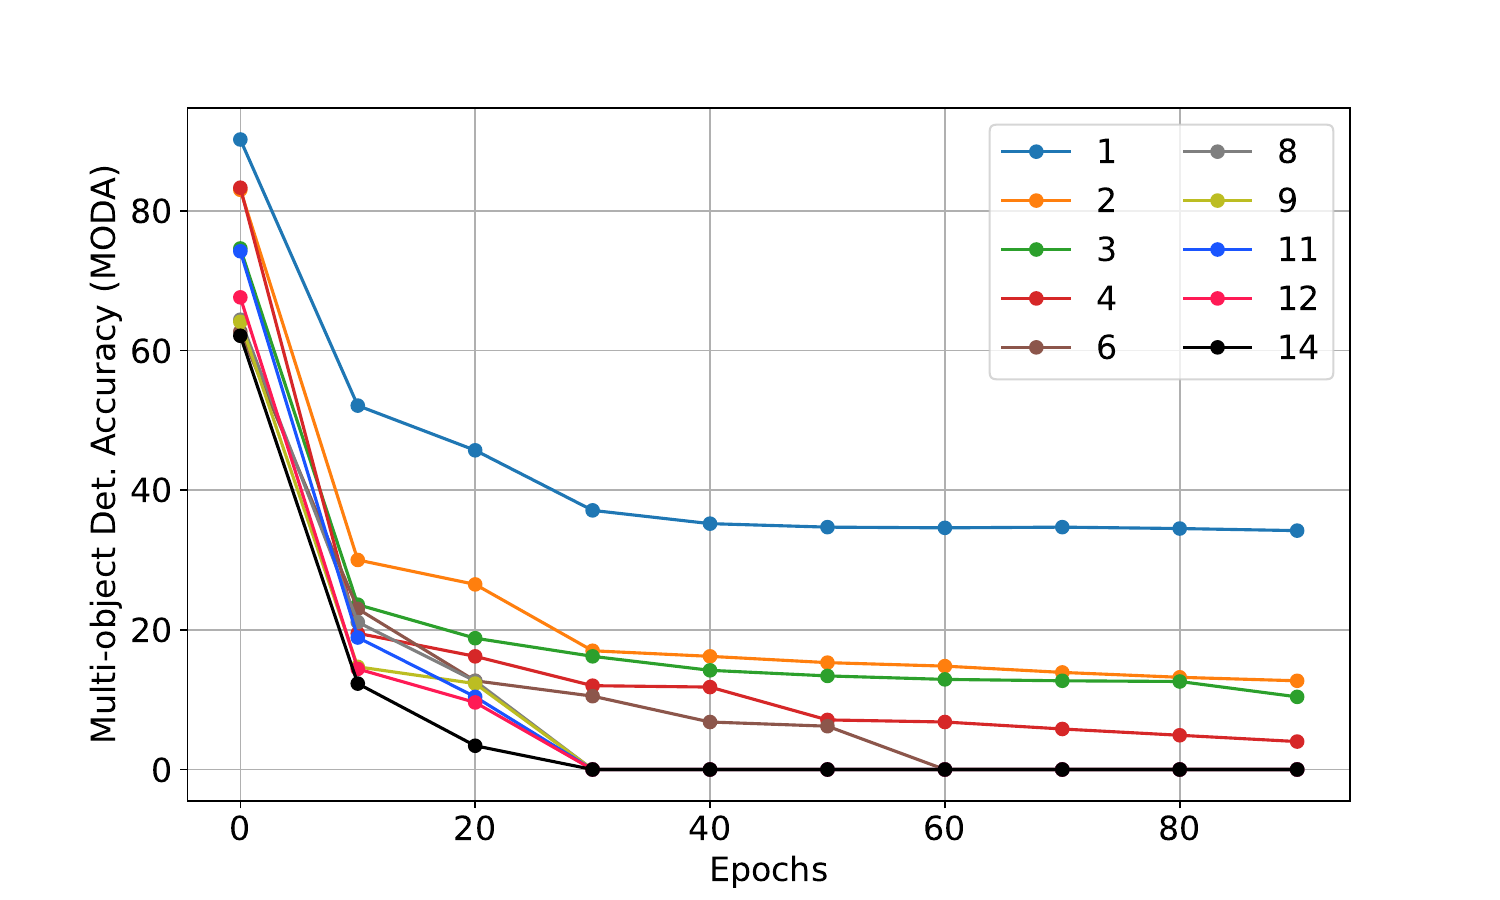}
    \caption{Training curve for increasing number of target patches}
    \label{fig:training-curve-num-tar}
\end{figure}

\subsection{Training curves for increasing adversarial cameras}
For this experiment, we choose the CP attack on MVDeTr, as MVDeTr can have multiple camera views. In Fig. \ref{fig:training-curve-num_cam} we see that with increasing number of adversarial cameras (cameras hosting source and/or target patches) the attack converges faster. In this experiment, as we added adversarial cameras, we added one source patch and one target patch, both of size 32x32.

\begin{figure}[h]
    \centering
    \includegraphics[width=\linewidth]{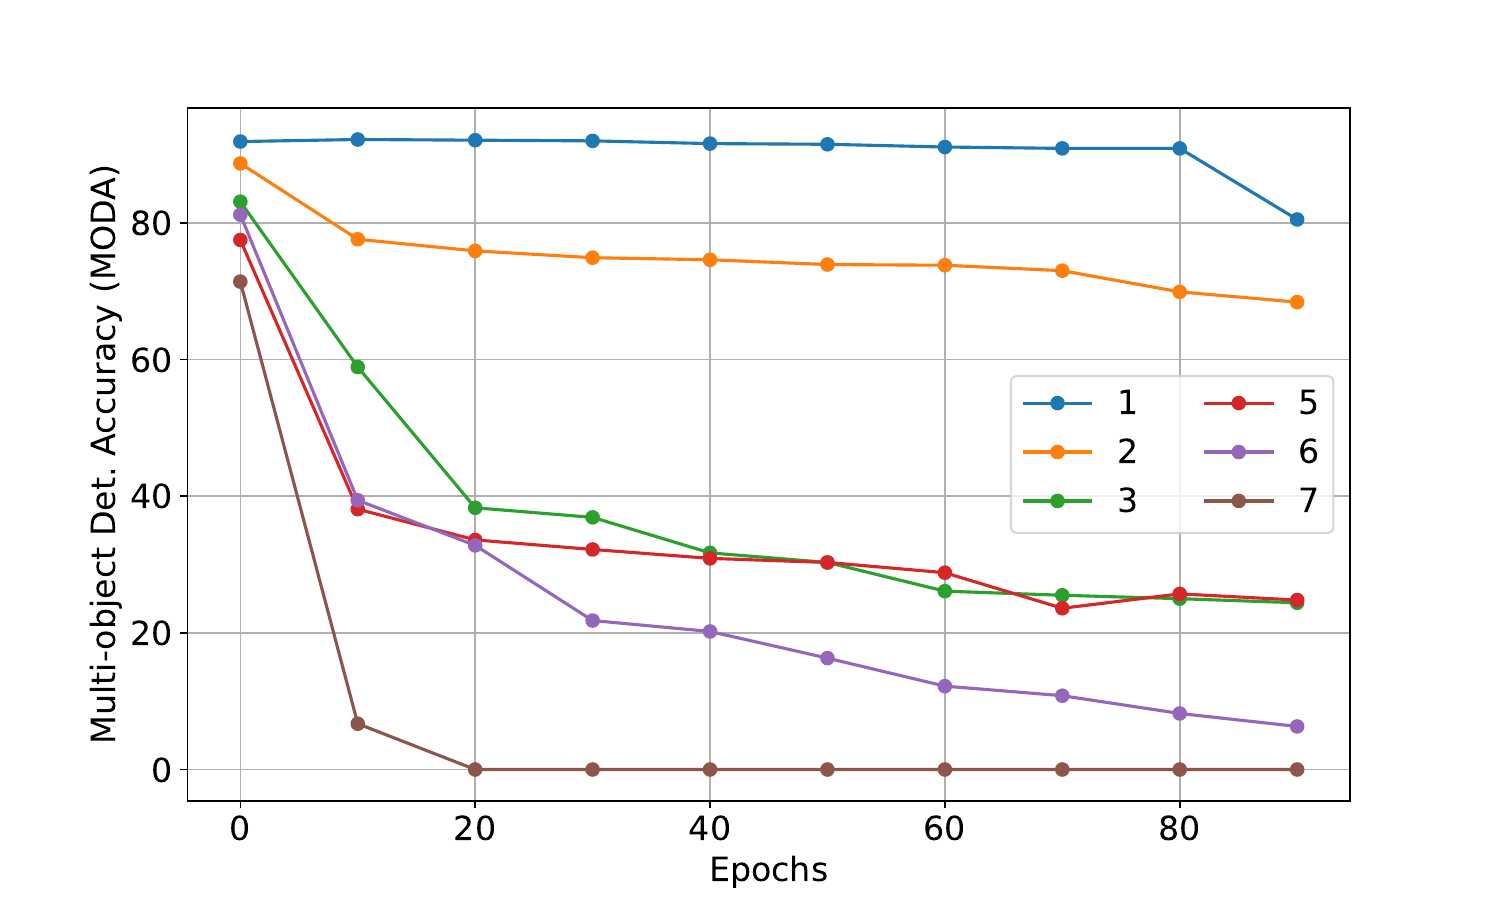}
    \caption{Training curve for increasing number of adversarial camera}
    \label{fig:training-curve-num_cam}
\end{figure}
